# Supplementary material for: Do Encoder Representations of Generative Dialogue Models Encode Sufficient Information about the Task ?
Source: arXiv:2106.10622 source file (2021-06-20)
Supplement: Supplementary file 2 [file arXiv_appendix.tex]

\section*{Appendix}
\section{Model Parameters}
\begin{table}
    \centering
    \small
    \begin{tabular}{p{5cm}|c}
    \hline
       {\bf Model}  & {\bf Parameters}  \\
    \hline
        \rowcolor{Gray}{\it LSTM Encoder-Decoder} &	11M \\
        {\it LSTM Encoder-Decoder + Attention} &	11M \\
        \rowcolor{Gray}{\it HRED} &	12M \\
        {\it Bi-LSTM Encoder-Decoder}	& 12M\\
        \rowcolor{Gray}{\it Transformer}	& 41M \\
    \hline
    \end{tabular}
    \caption{Size of parameters of the models used in all the experiments on the two data sets. \emph{M} for Million.}
    \label{tab:size-of-models}
\end{table}

\label{sec:model-parameters}
\begin{itemize}
    \item For SEQ2SEQ models, we used a 256 unit hidden size LSTM with 2 layers and a 128 unit input embedding dimension. The learning rate we used for all the models is 4E-3. 
    \item For Transformer, we used a 512 unit hidden size, 512 unit input embedding dimension, 2 attention header and 4 layers. 
    \item We used Adam as the optimizer to optimize on the cross-entropy loss. 
    \item We averaged the results over 3 different seeds.
    \item We used a truncated history of last 100 tokens as context to keep the training uniform across the models.
\end{itemize}

\section{Data Preparation}
\label{sec:data-preparation}
\subsection{MultiWoZ}
We use the minimal information in the annotated json dataset to add additional details to the dialogue state. The annotation has texts of user and agent utterances with slot and value pairs parsed from the user utterance. We parse and process the slot-value pairs data into information like task topics, recent slot, among others used in the probe tasks. For UtteranceLoc, we bucket the utterances based on the position they occur in a conversation.

\subsection{PersonaChat}
PersonaChat dataset has persona details along with text utterances from two different users. We extract only the non-stop words from the persona information for PersonalInfo task. For WordCont, we order the vocab descending frequency and select 500 words that occur for 1000-3000 times in the dataset.

\section{Distribution of Information}
\label{sec:information-distribution}
Before creating the probe tasks to test the model, we wanted to ensure that the outputs of the tasks have a spread out distribution over the outputs such that the model can be evaluated on its understanding with the probe tasks. The distributional analysis on MultiWoZ data is shown in Figure \ref{fig:distribution-multiwoz} suggests that in addition to diversity in token level there is diversity in the underlying information which charcterizes the response. 

\begin{figure*}[h!]
\centering
\subfigure[Distribution of Topics]{
    \includegraphics[width=0.8\columnwidth]{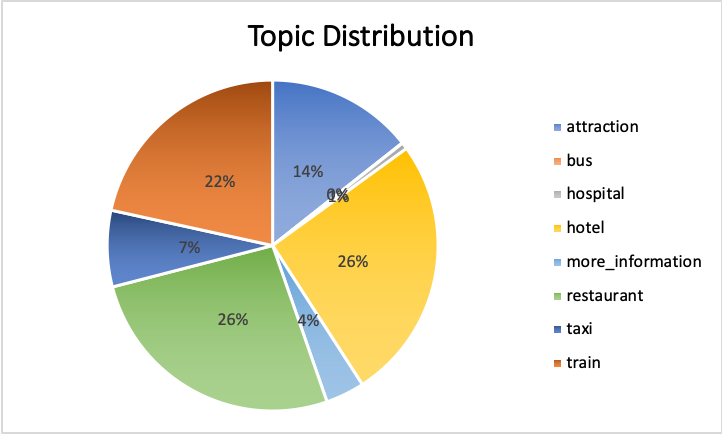}
}
\subfigure[\#Topics Distribution in a Conversation]{
    \includegraphics[width=0.8\columnwidth]{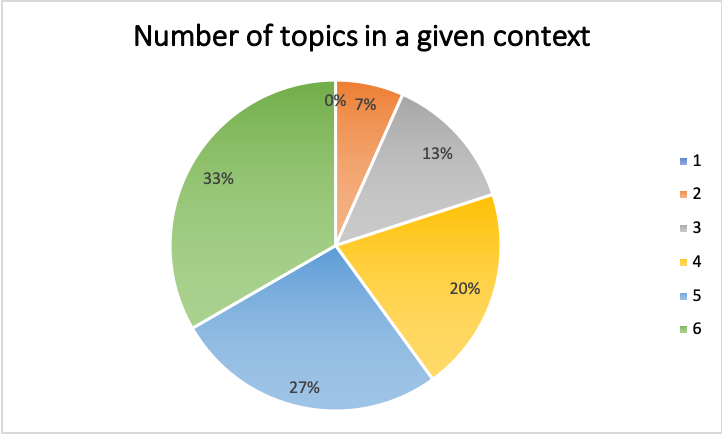}
}
\\
\subfigure[Number of Information in Single Utterance]{
    \includegraphics[width=0.8\columnwidth]{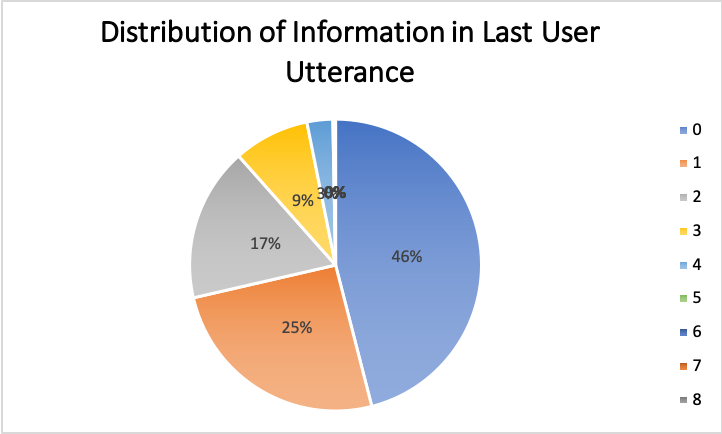}
}
\subfigure[Number of information Repeating in a Context]{
    \includegraphics[width=0.8\columnwidth]{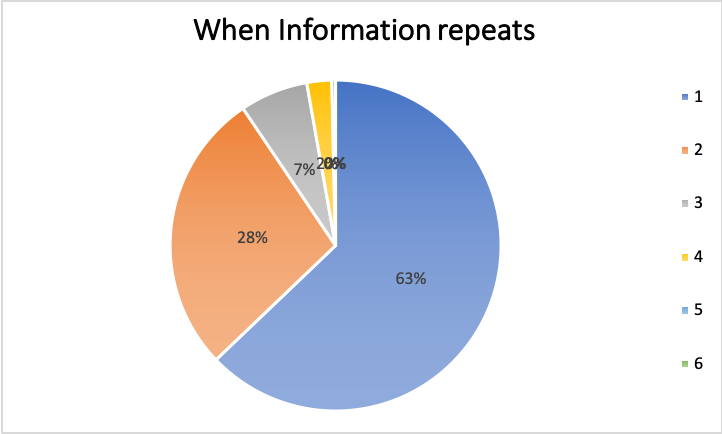}
}
\\
\subfigure[Distribution of Single and Multiple Tasks]{
    \includegraphics[width=0.8\columnwidth]{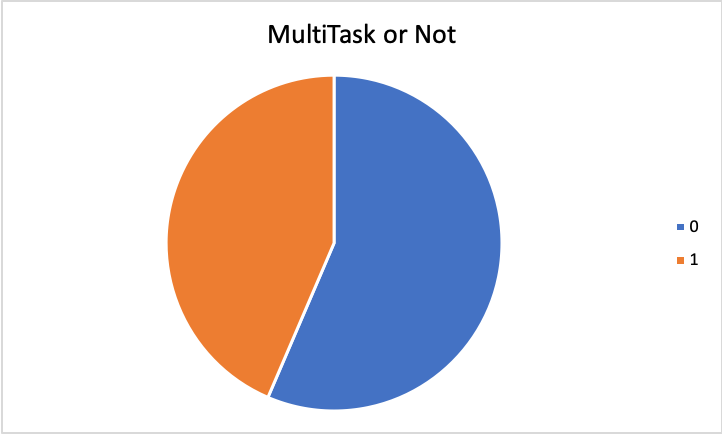}
}
\subfigure[Location of Utterance Distribution]{
    \includegraphics[width=0.8\columnwidth]{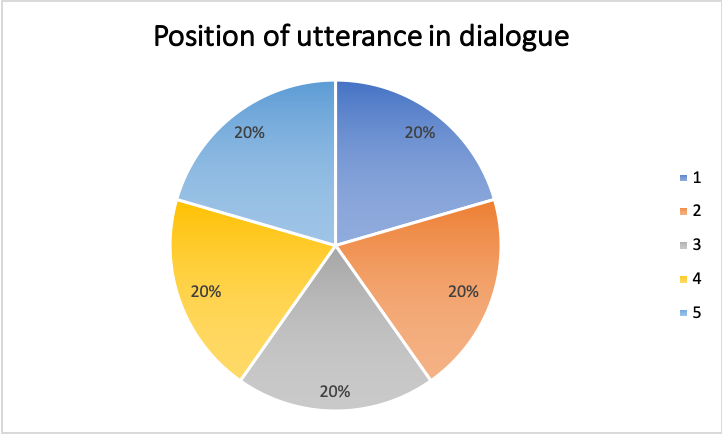}
}
\\
\subfigure[Response Length Distribution]{
    \includegraphics[width=0.8\columnwidth]{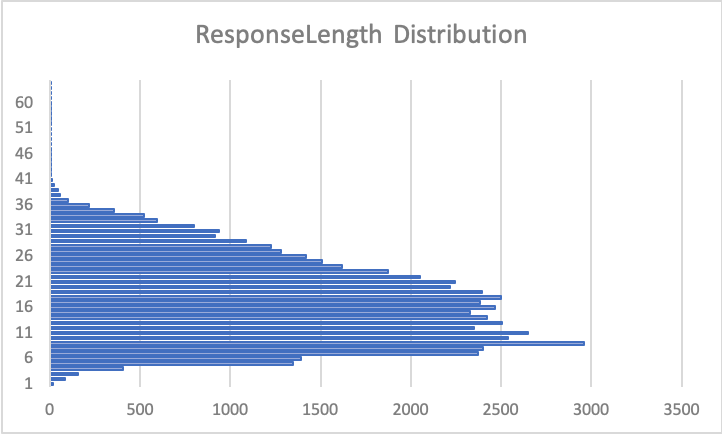}
}
\subfigure[Distribution of information load in dialogues]{
    \includegraphics[width=0.8\columnwidth]{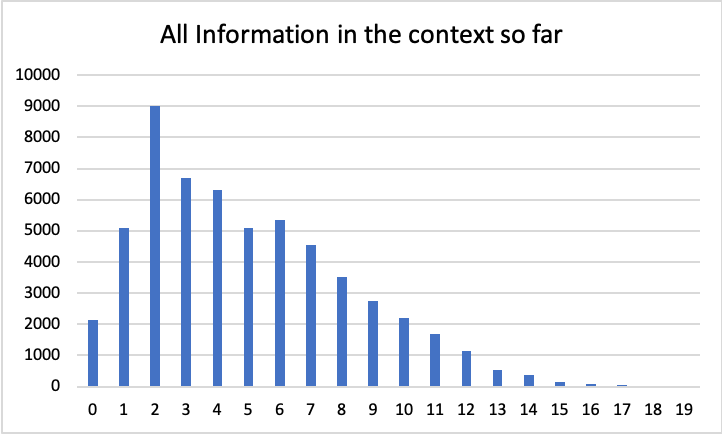}
}
\caption{Analysis of information available through probe tasks on MultiWoZ dialogue dataset.}
\label{fig:distribution-multiwoz}
\end{figure*}
To that end, we create probe tasks with the annotated information extracted from the dataset to evaluate the understanding of the dialogue architectures.

\section{Additional Experiments}
\label{sec:addn-experiments}
Similar to the encoder representation observed on the MultiWoZ dataset, we observed the encoder representation between the first and the last epoch with training on PersonaChat dataset. 
\begin{figure*}[!h]
\centering
\subfigure[Seq2Seq Model after 0 Epoch]{
    \includegraphics[width=0.8\columnwidth]{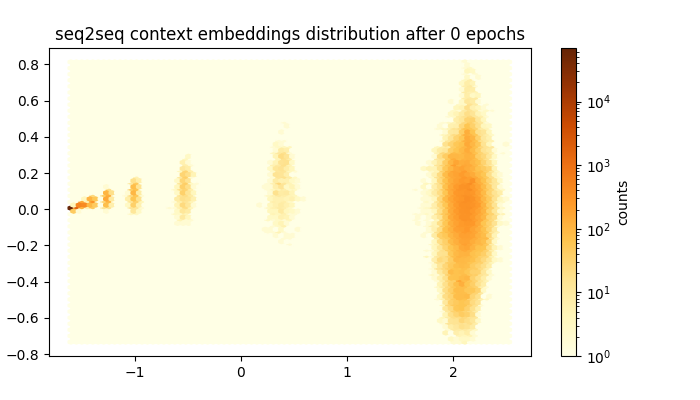}
}
\subfigure[Seq2Seq Model after Last Epoch]{
    \includegraphics[width=0.8\columnwidth]{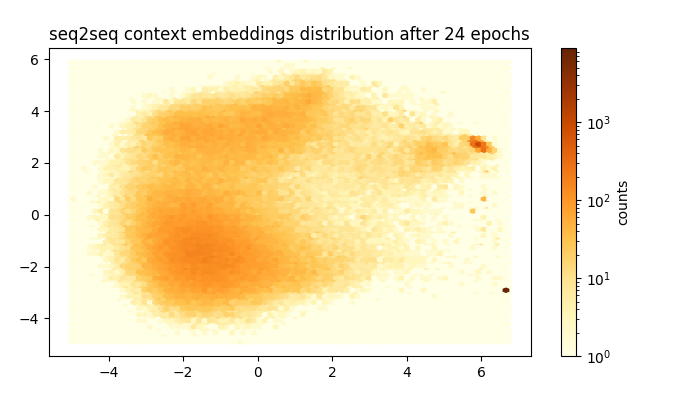}
}
\\
\subfigure[Seq2Seq Attention Model after 0 Epoch]{
    \includegraphics[width=0.8\columnwidth]{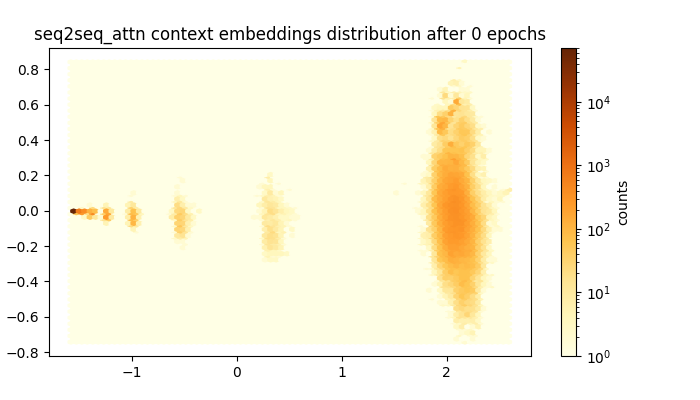}
}
\subfigure[Seq2Seq Attention Model after Last Epoch]{
    \includegraphics[width=0.8\columnwidth]{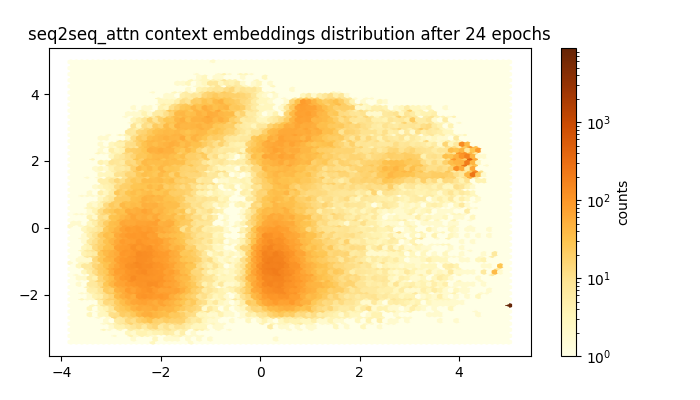}
}
\\
\subfigure[Bi-LSTM Attention Model after 0 Epoch]{
    \includegraphics[width=0.8\columnwidth]{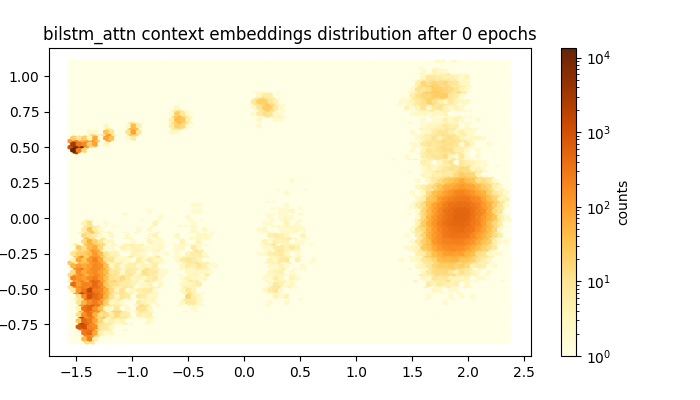}
}
\subfigure[Bi-LSTM Attention Model after Last Epoch]{
    \includegraphics[width=0.8\columnwidth]{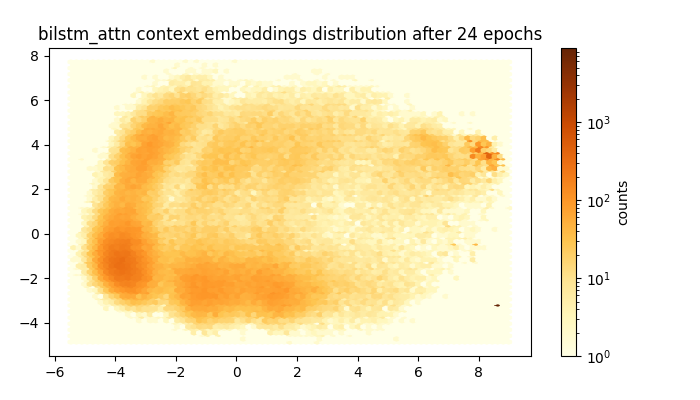}
}
\\
\subfigure[HRED Model after 0 Epoch]{
    \includegraphics[width=0.8\columnwidth]{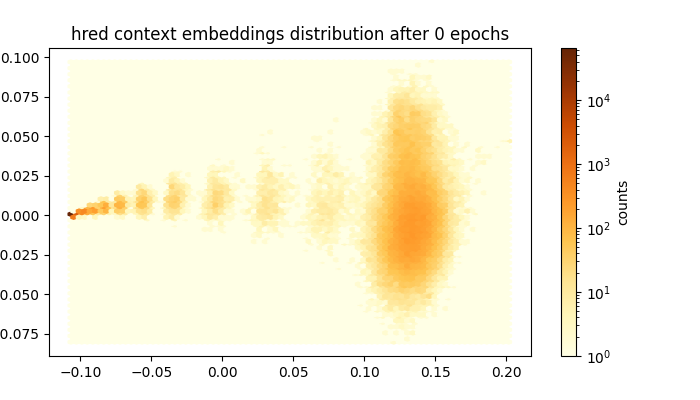}
}
\subfigure[HRED Model after Last Epoch]{
    \includegraphics[width=0.8\columnwidth]{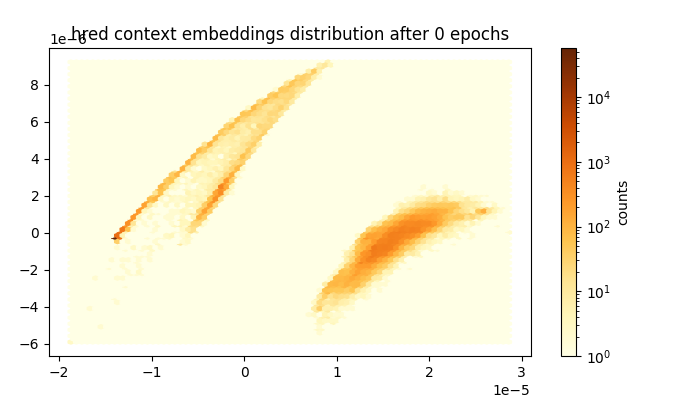}
}
\\
\subfigure[Transformer Model after 1 Epoch]{
    \includegraphics[width=0.8\columnwidth]{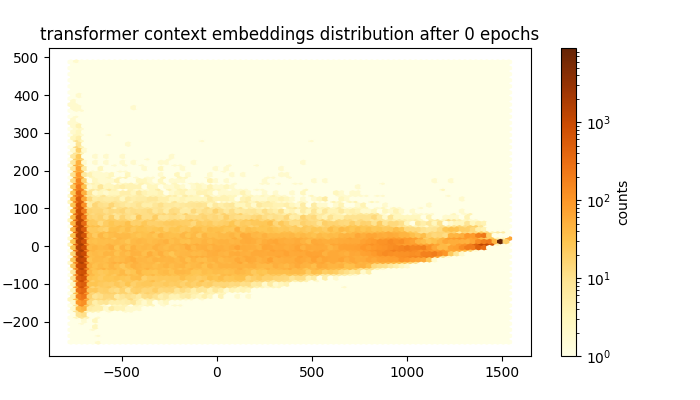}
}
\subfigure[Transformer Model after 24 Epoch]{
    \includegraphics[width=0.8\columnwidth]{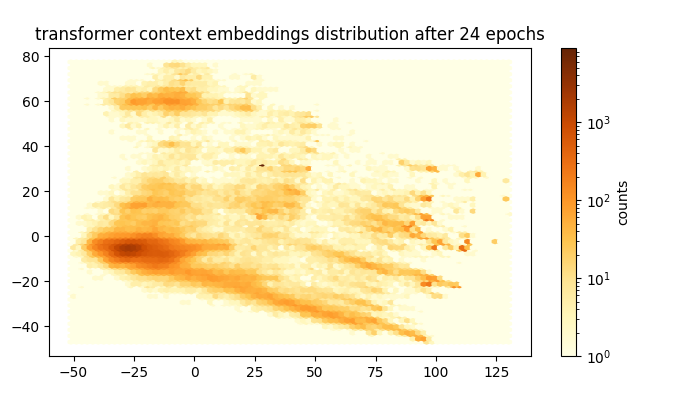}
}
\caption{Downsampled encoder hidden states on PersonaChat dataset by projecting on to two principal components. The encoder representation manifold shows that Transformer model has high capacity to encode a large dataset but not the SEQ2SEQ models.}
\label{fig:personachat-context}
\end{figure*}
PersonaChat dataset being an open-domain dialogue dataset, we did not observe strong tendency to cluster in the encoder representation. Non-existence of clusters shows that the model struggle to summarize the information available, explaining the lower performance on BLEU score and probe tasks on the dataset. 

\subsection{Comparison of Model Selection on probe tasks}

We experimented on selecting models based with METEOR, ROUGE-F1(F1), Average vector with BERT encoding as alternate selection metric to BLEU on the two datasets Table \ref{tab:multiwoz-probe-tasks-1-metric},\ref{tab:multiwoz-probe-tasks-metric},\ref{tab:persona-probe-tasks-metric}. 
\begin{table}[h!]
\tiny
\centering
      \begin{tabular}{c|a|b|a}
         \hline
         \multicolumn{4}{c}{PersonaChat Dataset}\\
         \hline
         {\bf Model} & {\bf UtteranceLoc} & {\bf WordCont} & {\bf PersonalInfo} \\
         \hline
         \rowcolor{LightBlue}\multicolumn{4}{c}{Bi-LSTM Seq2Seq + Attention} \\
         \hline
         BERT &58.89 $\pm$ 0.02 &40.43 $\pm$ 0.02 &0.00 $\pm$ 0.00    \\
         F1 & 57.27 $\pm$ 0.02 &40.28 $\pm$ 0.06 &0.02 $\pm$ 0.00   \\
         BLEU & 57.19 $\pm$ 0.05 &39.72 $\pm$ 0.08 &0.02 $\pm$ 0.00   \\
         METEOR & 57.48 $\pm$ 0.04 &39.29 $\pm$ 0.01 &0.02 $\pm$ 0.00 \\
        \hline
         \rowcolor{LightBlue}\multicolumn{4}{c}{HRED - LSTM} \\
         \hline
         BERT & 0.00 $\pm$ 0.00 &51.97 $\pm$ 0.01 &0.00 $\pm$ 0.00 \\
         F1 &0.00 $\pm$ 0.00 &51.97 $\pm$ 0.01 &0.00 $\pm$ 0.00  \\
         BLEU & 10.76 $\pm$ 3.48 &51.00 $\pm$ 0.07 &0.00 $\pm$ 0.00  \\
         METEOR & 0.00 $\pm$ 0.00 &51.97 $\pm$ 0.01 &0.00 $\pm$ 0.00 \\
         \hline
         \rowcolor{LightBlue}\multicolumn{4}{c}{LSTM Seq2Seq + Attention} \\
         \hline
         BERT & 55.12 $\pm$ 0.04 &42.04 $\pm$ 0.03 &0.00 $\pm$ 0.00  \\
         F1 & 48.11 $\pm$ 0.48 &41.84 $\pm$ 0.08 &0.01 $\pm$ 0.00  \\
         BestBLEU & 54.06 $\pm$ 0.06 &43.77 $\pm$ 0.24 &0.00 $\pm$ 0.00  \\
         METEOR & 51.91 $\pm$ 0.00 &42.36 $\pm$ 0.13 &0.00 $\pm$ 0.00 \\
         \hline
         \rowcolor{LightBlue}\multicolumn{4}{c}{LSTM Seq2Seq} \\
         \hline
         BERT & 50.32 $\pm$ 0.90 &42.99 $\pm$ 0.04 &0.00 $\pm$ 0.00   \\
         F1 & 52.23 $\pm$ 0.09 &39.98 $\pm$ 0.02 &0.01 $\pm$ 0.00    \\
         BLEU & 52.23 $\pm$ 0.08 &40.16 $\pm$ 0.04 &0.01 $\pm$ 0.00  \\
         METEOR & 52.17 $\pm$ 0.11 &40.54 $\pm$ 0.00 &0.01 $\pm$ 0.00\\
         \hline
         \rowcolor{LightBlue}\multicolumn{4}{c}{Transformer Architecture} \\
         \hline
         BERT & 42.30 $\pm$ 0.02 &45.71 $\pm$ 0.12 &0.02 $\pm$ 0.00 \\
         F1 & 40.33 $\pm$ 0.07 &47.15 $\pm$ 0.06 &0.00 $\pm$ 0.00 \\
         BLEU & 40.73 $\pm$ 0.06 &46.16 $\pm$ 0.03 &0.03 $\pm$ 0.00 \\
         METEOR & 39.73 $\pm$ 0.02 &45.76 $\pm$ 0.07 &0.01 $\pm$ 0.00 \\
         \hline
    \end{tabular}
    \caption{Comparison of models selected different selection metrics on probe tasks in PersonaChat dialogue data set. The performance is measured with \emph{F1} on the probetasks.}
    \label{tab:persona-probe-tasks-metric}
\end{table}

 \begin{table*}[h!]
        \tiny
        \centering
        \begin{tabular}{c|a|b|a|b|a|b|a|b}
         \hline
         \multicolumn{9}{c}{MultiWoZ Dataset}\\
         \hline
         {\bf Model} & {\bf UtteranceLoc} & {\bf RecentTopic} & {\bf RecentSlots} & {\bf RecentValues} & {\bf RepeatInfo} & {\bf NumRepeatInfo}& {\bf NumRecentInfo} & {\bf AllSlots} \\
         \hline
         \rowcolor{LightBlue}\multicolumn{9}{c}{LSTM Seq2Seq + Attention} \\
         \hline
         BERT &37.12 $\pm$ 2.59 &42.74 $\pm$ 16.78 &43.53 $\pm$ 4.54 &30.93 $\pm$ 0.63 &70.82 $\pm$ 0.01 &74.71 $\pm$ 0.01 &44.76 $\pm$ 1.89 &23.94 $\pm$ 6.31 \\
         F1 &58.08 $\pm$ 0.09 &89.31 $\pm$ 0.08 &66.72 $\pm$ 0.02 &39.55 $\pm$ 0.05 &71.25 $\pm$ 0.01 &75.10 $\pm$ 0.00 &62.14 $\pm$ 0.02 &52.57 $\pm$ 0.10 \\
         BLEU & 57.55 $\pm$ 0.05 &89.91 $\pm$ 0.07 &67.39 $\pm$ 0.02 &40.49 $\pm$ 0.04 &70.92 $\pm$ 0.00 &74.73 $\pm$ 0.00 &62.48 $\pm$ 0.02 &53.08 $\pm$ 0.11 \\
         METEOR &58.23 $\pm$ 0.08 &89.26 $\pm$ 0.08 &66.83 $\pm$ 0.02 &39.72 $\pm$ 0.04 &71.29 $\pm$ 0.00 &75.01 $\pm$ 0.00 &62.23 $\pm$ 0.01 &52.58 $\pm$ 0.10\\
        \hline
         \rowcolor{LightBlue}\multicolumn{9}{c}{HRED - LSTM} \\
         \hline
         BERT &18.78 $\pm$ 10.58 &23.78 $\pm$ 16.97 &16.41 $\pm$ 8.07 &10.44 $\pm$ 3.27 &71.78 $\pm$ 0.02 &75.51 $\pm$ 0.01 &19.27 $\pm$ 11.14 &13.31 $\pm$ 5.31 \\
         F1 &37.18 $\pm$ 10.38 &49.59 $\pm$ 19.55 &33.95 $\pm$ 8.98 &20.81 $\pm$ 3.26 &71.33 $\pm$ 0.01 &74.99 $\pm$ 0.01 &38.49 $\pm$ 11.14 &28.49 $\pm$ 6.63 \\
         BLEU & 37.15 $\pm$ 10.35 &50.98 $\pm$ 20.94 &34.84 $\pm$ 9.69 &20.63 $\pm$ 3.21 &71.68 $\pm$ 0.00 &75.06 $\pm$ 0.00 &38.59 $\pm$ 11.18 &30.23 $\pm$ 7.84 \\
         METEOR &41.04 $\pm$ 5.85 &50.78 $\pm$ 20.86 &44.50 $\pm$ 2.49 &28.96 $\pm$ 0.18 &71.72 $\pm$ 0.00 &75.28 $\pm$ 0.00 &50.71 $\pm$ 1.44 &30.21 $\pm$ 7.84 \\
         \hline
         \rowcolor{LightBlue}\multicolumn{9}{c}{LSTM Seq2Seq } \\
         \hline
         BERT &54.16 $\pm$ 0.94 &63.24 $\pm$ 16.20 &55.13 $\pm$ 4.78 &34.62 $\pm$ 0.76 &72.00 $\pm$ 0.00 &75.90 $\pm$ 0.00 &54.06 $\pm$ 2.46 &37.48 $\pm$ 5.21  \\
         F1 &57.56 $\pm$ 0.06 &89.44 $\pm$ 0.04 &68.00 $\pm$ 0.00 &40.98 $\pm$ 0.03 &71.22 $\pm$ 0.01 &75.32 $\pm$ 0.01 &62.78 $\pm$ 0.01 &53.07 $\pm$ 0.04\\
         BLEU& 57.37 $\pm$ 0.06 &89.45 $\pm$ 0.03 &68.08 $\pm$ 0.01 &39.78 $\pm$ 0.07 &71.28 $\pm$ 0.01 &75.36 $\pm$ 0.01 &62.33 $\pm$ 0.05 &53.40 $\pm$ 0.05 \\
         METEOR & 57.84 $\pm$ 0.04 &89.03 $\pm$ 0.01 &67.74 $\pm$ 0.01 &40.37 $\pm$ 0.10 &71.10 $\pm$ 0.00 &74.75 $\pm$ 0.00 &61.85 $\pm$ 0.00 &53.04 $\pm$ 0.02 \\
         \hline
         \rowcolor{LightBlue}\multicolumn{9}{c}{Bi-LSTM Seq2Seq + Attention} \\
         \hline
         BERT & 57.98 $\pm$ 0.03 &78.79 $\pm$ 3.19 &57.24 $\pm$ 1.71 &35.59 $\pm$ 0.34 &71.35 $\pm$ 0.00 &75.18 $\pm$ 0.01 &57.57 $\pm$ 0.18 &48.37 $\pm$ 1.11\\
         F1 &57.99 $\pm$ 0.05 &89.63 $\pm$ 0.03 &64.85 $\pm$ 0.00 &39.16 $\pm$ 0.00 &71.76 $\pm$ 0.01 &75.30 $\pm$ 0.01 &60.85 $\pm$ 0.07 &54.68 $\pm$ 0.04  \\
         BLEU & 59.04 $\pm$ 0.10 &89.85 $\pm$ 0.03 &65.03 $\pm$ 0.00 &39.06 $\pm$ 0.00 &71.98 $\pm$ 0.01 &75.63 $\pm$ 0.00 &60.36 $\pm$ 0.05 &54.96 $\pm$ 0.05  \\
         METEOR &58.45 $\pm$ 0.07 &89.28 $\pm$ 0.02 &64.21 $\pm$ 0.00 &39.19 $\pm$ 0.00 &71.54 $\pm$ 0.00 &75.35 $\pm$ 0.01 &60.49 $\pm$ 0.05 &54.65 $\pm$ 0.04  \\
         \hline
         \rowcolor{LightBlue}\multicolumn{9}{c}{Transformer Architecture} \\
         \hline
         BERT &39.11 $\pm$ 0.09 &58.38 $\pm$ 0.14 &29.97 $\pm$ 0.00 &24.50 $\pm$ 0.01 &72.39 $\pm$ 0.01 &76.02 $\pm$ 0.00 &38.80 $\pm$ 0.01 &43.37 $\pm$ 0.17 \\
         F1 & 39.89 $\pm$ 0.21 &67.44 $\pm$ 0.44 &33.37 $\pm$ 0.14 &24.96 $\pm$ 0.02 &72.75 $\pm$ 0.01 &76.26 $\pm$ 0.00 &40.43 $\pm$ 0.05 &51.19 $\pm$ 0.51\\
         BLEU &39.46 $\pm$ 0.00 &57.05 $\pm$ 1.50 &30.10 $\pm$ 0.27 &23.72 $\pm$ 0.03 &72.70 $\pm$ 0.00 &75.97 $\pm$ 0.00 &39.11 $\pm$ 0.08 &40.43 $\pm$ 1.21\\
         METEOR &38.50 $\pm$ 0.25 &56.26 $\pm$ 1.87 &30.98 $\pm$ 0.11 &24.94 $\pm$ 0.02 &72.26 $\pm$ 0.01 &75.79 $\pm$ 0.00 &39.47 $\pm$ 0.04 &38.70 $\pm$ 1.59\\
         \hline
    \end{tabular}
    \caption{Comparison of models selected different selection metrics on probe tasks in MultiWoZ dialogue data set. The performance is measured with \emph{F1} on the probetasks.}
    \label{tab:multiwoz-probe-tasks-1-metric}
\end{table*}

\begin{table*}[h!]
\tiny
\centering
    \begin{tabular}{c|a|b|a|b|a|b|a|b}
         \hline
         \multicolumn{9}{c}{MultiWoZ Dataset}\\
         \hline
         {\bf Metric} & {\bf AllValues} & {\bf NumAllInfo} & {\bf AllTopics}&{\bf NumAllTopics} & {\bf IsMultiTask} & {\bf EntitySlots} & {\bf EntityValues} & {\bf ActionSelect} \\
         \hline
         \rowcolor{LightBlue}\multicolumn{9}{c}{LSTM Seq2Seq + Attention} \\
         \hline
         BERT & 6.16 $\pm$ 0.34 &8.52 $\pm$ 2.18 &49.07 $\pm$ 5.13 &77.98 $\pm$ 0.00 &84.97 $\pm$ 0.01 &27.49 $\pm$ 1.30 &22.22 $\pm$ 0.47 &30.25 $\pm$ 6.74  \\
         F1 &12.54 $\pm$ 0.01 &26.54 $\pm$ 0.02 &75.22 $\pm$ 0.03 &79.56 $\pm$ 0.02 &84.70 $\pm$ 0.01 &41.74 $\pm$ 0.02 &31.20 $\pm$ 0.03 &60.00 $\pm$ 0.00\\
         BestBLEU  &12.81 $\pm$ 0.01 &25.73 $\pm$ 0.02 &75.33 $\pm$ 0.02 &79.39 $\pm$ 0.02 &85.30 $\pm$ 0.00 &41.29 $\pm$ 0.03 &31.57 $\pm$ 0.03 &60.14 $\pm$ 0.01\\
         METEOR & 12.53 $\pm$ 0.01 &26.62 $\pm$ 0.02 &75.21 $\pm$ 0.03 &79.52 $\pm$ 0.02 &84.67 $\pm$ 0.01 &41.70 $\pm$ 0.02 &31.48 $\pm$ 0.02 &60.06 $\pm$ 0.00 \\
        \hline
         \rowcolor{LightBlue}\multicolumn{9}{c}{HRED - LSTM} \\
         \hline
         BERT & 3.20 $\pm$ 0.31 &7.49 $\pm$ 1.68 &21.92 $\pm$ 14.41 &58.94 $\pm$ 3.05 &62.30 $\pm$ 4.46 &10.85 $\pm$ 3.53 &9.06 $\pm$ 2.46 &17.04 $\pm$ 8.72 \\
         F1 & 6.40 $\pm$ 0.32 &16.07 $\pm$ 1.97 &45.79 $\pm$ 16.07 &69.01 $\pm$ 3.62 &73.72 $\pm$ 4.79 &23.39 $\pm$ 4.22 &19.53 $\pm$ 2.87 &35.39 $\pm$ 9.73\\
         BLEU  & 6.90 $\pm$ 0.39 &14.96 $\pm$ 1.77 &46.63 $\pm$ 16.93 &68.66 $\pm$ 3.50 &72.97 $\pm$ 4.50 &24.33 $\pm$ 4.64 &19.97 $\pm$ 3.01 &35.66 $\pm$ 9.95\\
         METEOR & 6.82 $\pm$ 0.38 &15.93 $\pm$ 1.93 &54.09 $\pm$ 8.47 &79.20 $\pm$ 0.02 &85.55 $\pm$ 0.01 &30.35 $\pm$ 1.29 &25.88 $\pm$ 0.51 &36.00 $\pm$ 9.70 \\
         \hline
         \rowcolor{LightBlue}\multicolumn{9}{c}{LSTM Seq2Seq } \\
         \hline
         BERT &9.16 $\pm$ 0.27 &18.10 $\pm$ 2.47 &60.55 $\pm$ 4.58 &77.91 $\pm$ 0.03 &84.43 $\pm$ 0.02 &34.68 $\pm$ 1.90 &27.23 $\pm$ 0.79 &45.12 $\pm$ 7.11\\
         F1  & 12.92 $\pm$ 0.01 &26.47 $\pm$ 0.04 &74.63 $\pm$ 0.03 &78.44 $\pm$ 0.00 &84.05 $\pm$ 0.01 &43.66 $\pm$ 0.01 &31.83 $\pm$ 0.01 &61.11 $\pm$ 0.01 \\
         BLEU  &12.76 $\pm$ 0.01 &26.94 $\pm$ 0.04 &75.03 $\pm$ 0.03 &78.16 $\pm$ 0.00 &83.90 $\pm$ 0.00 &43.92 $\pm$ 0.01 &31.96 $\pm$ 0.01 &61.13 $\pm$ 0.00\\
         METEOR & 12.97 $\pm$ 0.00 &25.97 $\pm$ 0.03 &74.37 $\pm$ 0.01 &78.42 $\pm$ 0.00 &84.03 $\pm$ 0.01 &43.79 $\pm$ 0.04 &31.63 $\pm$ 0.02 &61.22 $\pm$ 0.02 \\
         \hline
         \rowcolor{LightBlue}\multicolumn{9}{c}{Bi-LSTM Seq2Seq + Attention} \\
         \hline
         BERT & 12.83 $\pm$ 0.10 &23.74 $\pm$ 0.13 &71.48 $\pm$ 1.07 &78.54 $\pm$ 0.07 &85.60 $\pm$ 0.00 &35.96 $\pm$ 0.72 &26.88 $\pm$ 0.07 &50.57 $\pm$ 1.36  \\
         F1 & 14.92 $\pm$ 0.00 &26.67 $\pm$ 0.07 &78.01 $\pm$ 0.01 &81.02 $\pm$ 0.06 &86.17 $\pm$ 0.00 &40.61 $\pm$ 0.00 &29.38 $\pm$ 0.01 &57.91 $\pm$ 0.01 \\
         BLEU & 15.13 $\pm$ 0.01 &25.87 $\pm$ 0.05 &78.11 $\pm$ 0.02 &80.43 $\pm$ 0.02 &86.20 $\pm$ 0.00 &40.82 $\pm$ 0.01 &29.91 $\pm$ 0.02 &57.76 $\pm$ 0.00 \\
         METEOR & 14.81 $\pm$ 0.00 &26.53 $\pm$ 0.07 &78.04 $\pm$ 0.01 &80.02 $\pm$ 0.01 &86.25 $\pm$ 0.00 &41.02 $\pm$ 0.00 &30.11 $\pm$ 0.02 &57.90 $\pm$ 0.01\\
         \hline
         \rowcolor{LightBlue}\multicolumn{9}{c}{Transformer Architecture} \\
         \hline
         BERT  & 11.81 $\pm$ 0.04 &9.01 $\pm$ 0.06 &65.01 $\pm$ 0.09 &76.23 $\pm$ 0.02 &84.38 $\pm$ 0.01 &20.60 $\pm$ 0.00 &18.87 $\pm$ 0.02 &15.48 $\pm$ 0.14 \\
         F1  & 17.97 $\pm$ 0.64 &11.26 $\pm$ 0.17 &71.08 $\pm$ 0.24 &77.82 $\pm$ 0.03 &85.27 $\pm$ 0.01 &22.47 $\pm$ 0.02 &19.06 $\pm$ 0.03 &20.24 $\pm$ 0.34 \\
         BestBLEU  & 10.43 $\pm$ 0.14 &9.71 $\pm$ 0.00 &64.42 $\pm$ 0.88 &76.10 $\pm$ 0.07 &84.20 $\pm$ 0.01 &19.83 $\pm$ 0.00 &18.34 $\pm$ 0.03 &15.35 $\pm$ 0.54\\
         METEOR & 10.77 $\pm$ 0.37 &7.92 $\pm$ 0.11 &63.64 $\pm$ 0.80 &76.58 $\pm$ 0.05 &84.50 $\pm$ 0.01 &20.17 $\pm$ 0.06 &18.38 $\pm$ 0.01 &15.03 $\pm$ 0.72\\
         \hline
    \end{tabular}
    \caption{Comparison of models selected different selection metrics on probe tasks in MultiWoZ dialogue data set. The performance is measured with \emph{F1} on the probetasks.}
    \label{tab:multiwoz-probe-tasks-metric}
\end{table*}
We compared the performance of these models on the probe tasks to understand if there is any correlation between the metric and higher performance on the probe tasks. But, we did not find any meaningful correlation between the scores and selection metric.

\subsection{Analysis of Non-linear Probing}
We experimented with multi-layer perceptron with ReLU non-linearity to analyze the trend in the model performance on the probing-tasks on the two different datasets in Tables \ref{tab:non-linear-multiwoz-probe-tasks-1},\ref{tab:non-linear-multiwoz-probe-tasks},\ref{tab:non-linear-persona-probe-tasks-metric}. Although there was some difference in the performance of individual probe tasks, the global trend of SEQ2SEQ models' performance improving with epochs while Transformer's performance decreasing with epochs remained constant. 

 \begin{table}[h!]
\tiny
\centering
      \begin{tabular}{c|a|b|a}
         \hline
         \multicolumn{4}{c}{PersonaChat Dataset}\\
         \hline
         {\bf Model} & {\bf UtteranceLoc} & {\bf WordCont} & {\bf PersonalInfo} \\
         \hline
         \rowcolor{LightBlue}\multicolumn{4}{c}{Bi-LSTM Seq2Seq + Attention} \\
         \hline
         Untrained & 38.61 $\pm$ 0.00 &39.76 $\pm$ 0.03 &0.61 $\pm$ 0.00\\
         LastEpoch & 59.05 $\pm$ 0.08 &35.82 $\pm$ 0.05 &1.29 $\pm$ 0.00  \\
         BestBLEU & 57.50 $\pm$ 0.01 &36.06 $\pm$ 0.05 &1.43 $\pm$ 0.00   \\
        \hline
         \rowcolor{LightBlue}\multicolumn{4}{c}{HRED - LSTM} \\
         \hline
         Untrained & 38.20 $\pm$ 0.03 &50.91 $\pm$ 0.08 &0.00 $\pm$ 0.00\\
         LastEpoch & 11.74 $\pm$ 4.13 &51.73 $\pm$ 0.02 &0.00 $\pm$ 0.00   \\
         BestBLEU & 12.41 $\pm$ 4.62 &51.97 $\pm$ 0.01 &0.00 $\pm$ 0.00  \\
         \hline
         \rowcolor{LightBlue}\multicolumn{4}{c}{LSTM Seq2Seq + Attention} \\
         \hline
         Untrained & 38.47 $\pm$ 1.21 &43.41 $\pm$ 0.02 &0.67 $\pm$ 0.00 \\
         LastEpoch & 52.45 $\pm$ 0.03 &34.16 $\pm$ 0.09 &1.15 $\pm$ 0.00 \\
         BestBLEU & 49.73 $\pm$ 0.23 &28.05 $\pm$ 1.78 &0.88 $\pm$ 0.01   \\
         \hline
         \rowcolor{LightBlue}\multicolumn{4}{c}{LSTM Seq2Seq} \\
         \hline
         Untrained & 44.18 $\pm$ 0.03 &43.08 $\pm$ 0.01 &0.74 $\pm$ 0.00\\
         LastEpoch & 51.23 $\pm$ 0.07 &36.12 $\pm$ 0.01 &1.07 $\pm$ 0.00  \\
         BestBLEU & 54.54 $\pm$ 0.02 &34.75 $\pm$ 0.03 &1.33 $\pm$ 0.00   \\
         \hline
         \rowcolor{LightBlue}\multicolumn{4}{c}{Transformer Architecture} \\
         \hline
         Untrained & 64.04 $\pm$ 0.01 &31.19 $\pm$ 0.77 &1.17 $\pm$ 0.00 \\
         LastEpoch & 51.74 $\pm$ 0.00 &47.99 $\pm$ 0.58 &0.00 $\pm$ 0.00 \\
         BestBLEU & 51.77 $\pm$ 0.00 &39.22 $\pm$ 4.09 &0.01 $\pm$ 0.00  \\
         \hline
    \end{tabular}
    \caption{Comparison of models on probe tasks in PersonaChat dialogue data set with a multi-layer perceptron on the different encoder representation. The performance is measured with \emph{F1} on the probetasks. The trend in the performance of the models is similar to with Logistic Regression, where the performance on WordCont task decreases with increase in training epochs, and the PersonalInfo task is still difficult for the models.}
    \label{tab:non-linear-persona-probe-tasks-metric}
\end{table}
  \begin{table*}[h!]
        \tiny
        \centering
        \begin{tabular}{c|a|b|a|b|a|b|a|b}
         \hline
         \multicolumn{9}{c}{MultiWoZ Dataset}\\
         \hline
         {\bf Model} & {\bf UtteranceLoc} & {\bf RecentTopic} & {\bf RecentSlots} & {\bf RecentValues} & {\bf RepeatInfo} & {\bf NumRepeatInfo}& {\bf NumRecentInfo} & {\bf AllSlots} \\
         \hline
         \rowcolor{LightBlue}\multicolumn{9}{c}{LSTM Seq2Seq + Attention} \\
         \hline
         Untrained &46.47 $\pm$ 0.49 &35.34 $\pm$ 0.00 &39.04 $\pm$ 0.01 &30.82 $\pm$ 0.00 &64.23 $\pm$ 0.02 &68.95 $\pm$ 0.01 &41.40 $\pm$ 0.03 &30.21 $\pm$ 0.00  \\
         LastEpoch &56.50 $\pm$ 0.06 &87.11 $\pm$ 0.01 &65.61 $\pm$ 0.00 &42.19 $\pm$ 0.00 &64.91 $\pm$ 0.00 &70.03 $\pm$ 0.01 &61.74 $\pm$ 0.06 &51.51 $\pm$ 0.01 \\
         BestBLEU &58.03 $\pm$ 0.05 &88.95 $\pm$ 0.04 &66.53 $\pm$ 0.00 &41.09 $\pm$ 0.01 &64.47 $\pm$ 0.00 &66.89 $\pm$ 0.02 &63.37 $\pm$ 0.02 &52.02 $\pm$ 0.05 \\
        \hline
         \rowcolor{LightBlue}\multicolumn{9}{c}{HRED - LSTM} \\
         \hline
         Untrained & 45.28 $\pm$ 1.56 &32.90 $\pm$ 0.02 &41.20 $\pm$ 0.03 &31.69 $\pm$ 0.02 &70.98 $\pm$ 0.01 &74.85 $\pm$ 0.01 &40.65 $\pm$ 0.03 &19.79 $\pm$ 0.03 \\
         LastEpoch & 37.96 $\pm$ 10.86 &54.21 $\pm$ 22.63 &36.27 $\pm$ 10.10 &21.27 $\pm$ 3.41 &69.42 $\pm$ 0.06 &74.02 $\pm$ 0.02 &39.45 $\pm$ 11.67 &32.77 $\pm$ 8.39 \\
         BestBLEU & 38.71 $\pm$ 11.27 &50.10 $\pm$ 20.50 &34.27 $\pm$ 9.34 &20.45 $\pm$ 3.14 &70.98 $\pm$ 0.07 &74.53 $\pm$ 0.09 &39.29 $\pm$ 11.58 &30.26 $\pm$ 7.87 \\
         \hline
         \rowcolor{LightBlue}\multicolumn{9}{c}{LSTM Seq2Seq } \\
         \hline
         Untrained &46.56 $\pm$ 0.31 &35.85 $\pm$ 0.00 &39.68 $\pm$ 0.00 &32.03 $\pm$ 0.01 &64.82 $\pm$ 0.03 &69.18 $\pm$ 0.04 &42.98 $\pm$ 0.01 &29.49 $\pm$ 0.00 \\
         LastEpoch &54.95 $\pm$ 0.06 &87.64 $\pm$ 0.01 &66.04 $\pm$ 0.01 &41.94 $\pm$ 0.01 &66.11 $\pm$ 0.00 &69.84 $\pm$ 0.01 &61.03 $\pm$ 0.04 &51.63 $\pm$ 0.01 \\
         BestBLEU&56.27 $\pm$ 0.03 &88.57 $\pm$ 0.02 &66.88 $\pm$ 0.00 &41.55 $\pm$ 0.04 &65.89 $\pm$ 0.00 &70.20 $\pm$ 0.01 &62.62 $\pm$ 0.00 &52.61 $\pm$ 0.03 \\
         \hline
         \rowcolor{LightBlue}\multicolumn{9}{c}{Bi-LSTM Seq2Seq + Attention} \\
         \hline
         Untrained &44.26 $\pm$ 0.02 &50.65 $\pm$ 0.07 &35.26 $\pm$ 0.01 &27.27 $\pm$ 0.01 &64.58 $\pm$ 0.02 &70.55 $\pm$ 0.00 &39.93 $\pm$ 0.00 &36.67 $\pm$ 0.01 \\
         LastEpoch &57.21 $\pm$ 0.04 &86.66 $\pm$ 0.01 &63.29 $\pm$ 0.01 &38.17 $\pm$ 0.02 &66.55 $\pm$ 0.00 &70.76 $\pm$ 0.00 &60.23 $\pm$ 0.07 &53.36 $\pm$ 0.00 \\
         BestBLEU &57.47 $\pm$ 0.07 &88.98 $\pm$ 0.01 &64.54 $\pm$ 0.01 &39.56 $\pm$ 0.01 &68.48 $\pm$ 0.00 &72.19 $\pm$ 0.00 &62.34 $\pm$ 0.03 &56.02 $\pm$ 0.02 \\
         \hline
         \rowcolor{LightBlue}\multicolumn{9}{c}{Transformer Architecture} \\
         \hline
         Untrained &51.24 $\pm$ 0.04 &80.25 $\pm$ 0.03 &45.58 $\pm$ 0.01 &30.61 $\pm$ 0.01 &70.36 $\pm$ 0.02 &73.25 $\pm$ 0.00 &47.47 $\pm$ 0.03 &62.94 $\pm$ 0.01 \\
         LastEpoch & 33.73 $\pm$ 0.48 &32.14 $\pm$ 1.87 &26.17 $\pm$ 1.87 &22.11 $\pm$ 1.65 &70.75 $\pm$ 0.04 &74.63 $\pm$ 0.03 &33.64 $\pm$ 3.26 &21.25 $\pm$ 0.57 \\
         BestBLEU &31.96 $\pm$ 0.47 &31.69 $\pm$ 5.29 &29.64 $\pm$ 0.34 &25.34 $\pm$ 0.21 &72.16 $\pm$ 0.00 &75.90 $\pm$ 0.00 &37.77 $\pm$ 0.37 &22.75 $\pm$ 1.44 \\
         \hline
    \end{tabular}
    \caption{The performance of multi-layer perceptron over the encoder representation of different generative dialogue models on probe tasks in MultiWoZ dialogue data set . The performance is measured with \emph{F1}. The results, similar to the probe tasks with Logistic Regression, show that SEQ2SEQ models perform significantly better than Transformer model on the probe tasks, despite the models falling behind in BLEU score.}
    \label{tab:non-linear-multiwoz-probe-tasks-1}
\end{table*}

\begin{table*}[h!]
\tiny
\centering
    \begin{tabular}{c|a|b|a|b|a|b|a|b}
         \hline
         \multicolumn{9}{c}{MultiWoZ Dataset}\\
         \hline
         {\bf Model} & {\bf AllValues} & {\bf NumAllInfo} & {\bf AllTopics}&{\bf NumAllTopics} & {\bf IsMultiTask} & {\bf EntitySlots} & {\bf EntityValues} & {\bf ActionSelect} \\
         \hline
         \rowcolor{LightBlue}\multicolumn{9}{c}{LSTM Seq2Seq + Attention} \\
         \hline
         Untrained &12.63 $\pm$ 0.01 &6.97 $\pm$ 0.01 &45.10 $\pm$ 0.00 &70.27 $\pm$ 0.02 &80.06 $\pm$ 0.01 &28.04 $\pm$ 0.00 &19.63 $\pm$ 0.00 &28.66 $\pm$ 0.00 \\
         LastEpoch & 19.33 $\pm$ 0.00 &29.28 $\pm$ 0.03 &73.35 $\pm$ 0.00 &76.25 $\pm$ 0.03 &81.54 $\pm$ 0.04 &43.48 $\pm$ 0.02 &28.42 $\pm$ 0.00 &56.21 $\pm$ 0.01 \\
         BestBLEU  &18.65 $\pm$ 0.00 &29.16 $\pm$ 0.03 &74.34 $\pm$ 0.02 &76.93 $\pm$ 0.05 &82.12 $\pm$ 0.00 &42.55 $\pm$ 0.01 &29.09 $\pm$ 0.00 &56.88 $\pm$ 0.00 \\
        \hline
         \rowcolor{LightBlue}\multicolumn{9}{c}{HRED - LSTM} \\
         \hline
         Untrained & 5.28 $\pm$ 0.00 &0.00 $\pm$ 0.00 &37.51 $\pm$ 0.04 &77.57 $\pm$ 0.00 &84.24 $\pm$ 0.00 &24.86 $\pm$ 0.07 &19.01 $\pm$ 0.04 &27.26 $\pm$ 0.01 \\
         LastEpoch &8.73 $\pm$ 0.69 &19.05 $\pm$ 2.80 &48.66 $\pm$ 18.04 &69.23 $\pm$ 3.68 &73.51 $\pm$ 4.69 &27.07 $\pm$ 5.64 &20.22 $\pm$ 3.07 &38.76 $\pm$ 11.28 \\
         BestBLEU  &8.44 $\pm$ 0.78 &18.03 $\pm$ 2.63 &46.61 $\pm$ 16.88 &68.56 $\pm$ 3.48 &73.19 $\pm$ 4.58 &24.80 $\pm$ 4.94 &20.06 $\pm$ 3.02 &34.40 $\pm$ 9.31 \\
         \hline
         \rowcolor{LightBlue}\multicolumn{9}{c}{LSTM Seq2Seq } \\
         \hline
         Untrained &13.29 $\pm$ 0.00 &6.29 $\pm$ 0.02 &43.04 $\pm$ 0.01 &73.33 $\pm$ 0.01 &80.38 $\pm$ 0.05 &27.28 $\pm$ 0.01 &20.34 $\pm$ 0.00 &29.00 $\pm$ 0.01 \\
         LastEpoch  &19.48 $\pm$ 0.00 &28.80 $\pm$ 0.01 &72.84 $\pm$ 0.01 &75.74 $\pm$ 0.01 &81.22 $\pm$ 0.00 &44.00 $\pm$ 0.01 &30.72 $\pm$ 0.01 &56.67 $\pm$ 0.01 \\
         BestBLEU  &18.78 $\pm$ 0.00 &29.67 $\pm$ 0.02 &74.28 $\pm$ 0.03 &77.08 $\pm$ 0.03 &81.89 $\pm$ 0.00 &44.21 $\pm$ 0.00 &28.88 $\pm$ 0.03 &57.16 $\pm$ 0.02 \\
         \hline
         \rowcolor{LightBlue}\multicolumn{9}{c}{Bi-LSTM Seq2Seq + Attention} \\
         \hline
         Untrained &14.94 $\pm$ 0.00 &10.88 $\pm$ 0.08 &56.79 $\pm$ 0.00 &71.36 $\pm$ 0.01 &79.49 $\pm$ 0.01 &24.21 $\pm$ 0.00 &19.04 $\pm$ 0.01 &26.07 $\pm$ 0.02 \\
         LastEpoch &20.00 $\pm$ 0.00 &28.54 $\pm$ 0.01 &74.83 $\pm$ 0.01 &78.37 $\pm$ 0.01 &83.97 $\pm$ 0.00 &42.08 $\pm$ 0.00 &29.55 $\pm$ 0.02 &55.43 $\pm$ 0.01 \\
         BestBLEU & 20.03 $\pm$ 0.01 &29.56 $\pm$ 0.04 &77.37 $\pm$ 0.00 &79.06 $\pm$ 0.01 &84.21 $\pm$ 0.01 &41.62 $\pm$ 0.03 &28.21 $\pm$ 0.00 &56.53 $\pm$ 0.00 \\
         \hline
         \rowcolor{LightBlue}\multicolumn{9}{c}{Transformer Architecture} \\
         \hline
         Untrained  & 39.62 $\pm$ 0.00 &27.26 $\pm$ 0.03 &81.16 $\pm$ 0.00 &77.63 $\pm$ 0.00 &82.79 $\pm$ 0.00 &30.29 $\pm$ 0.02 &19.72 $\pm$ 0.11 &38.48 $\pm$ 0.19 \\
         LastEpoch  &5.11 $\pm$ 0.12 &11.48 $\pm$ 0.50 &47.65 $\pm$ 1.28 &71.93 $\pm$ 0.00 &82.00 $\pm$ 0.01 &13.48 $\pm$ 0.40 &13.35 $\pm$ 0.04 &6.76 $\pm$ 0.09\\
         BestBLEU  & 5.56 $\pm$ 0.14 &7.30 $\pm$ 0.23 &50.38 $\pm$ 1.14 &73.49 $\pm$ 0.04 &81.71 $\pm$ 0.01 &23.28 $\pm$ 0.14 &12.21 $\pm$ 0.33 &7.79 $\pm$ 0.22 \\
         \hline
    \end{tabular}
    \caption{The performance of different generative dialogue models on probe tasks in MultiWoZ dialogue data set. The performance is measured with $F-1$. The results show that SEQ2SEQ models show signs of learning on the probe tasks indirectly by learning to generate next utterance. Whereas the Transformer model's performance decreased from initial to last epoch in majority of the tasks.}
    \label{tab:non-linear-multiwoz-probe-tasks}
\end{table*}
\subsection{Performance Evolution on Probe Tasks}
Although we observed in Table \ref{tab:persona-probe-tasks} and \ref{tab:multiwoz-probe-tasks} that Transformer model architecture's performance decreasing while its BLEU score is higher in the task, we experimented to observe the evolution of the model performance on these probe tasks in Figures \ref{fig:probetasks_table1_multiwoz},\ref{fig:probetasks_table2_multiwoz} and \ref{fig:probetasks_table1_personachat}. We observed the trend in transformer in medium and hard probe tasks that its performance decreased and almost always stayed below the SEQ2SEQ models. This shows that the BLEU score and performance on probe tasks do not correlate, as inductive biases in a model can force the model to overfit to the patterns in text without actually understanding it.

\begin{figure*}[h!]
\centering
\subfigure[UtteranceLoc]{
    \includegraphics[width=0.8\columnwidth]{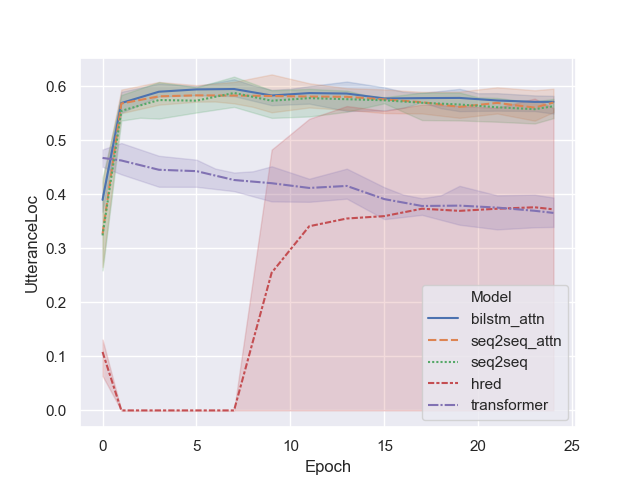}
}
\subfigure[RecentTopic]{
    \includegraphics[width=0.8\columnwidth]{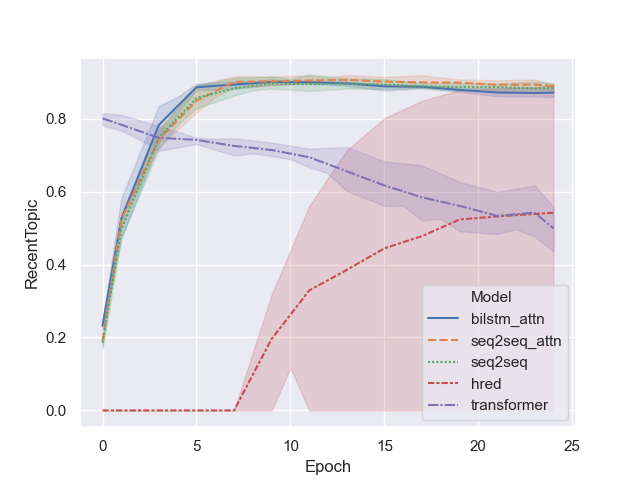}
}
\\
\subfigure[RecentSlots]{
    \includegraphics[width=0.8\columnwidth]{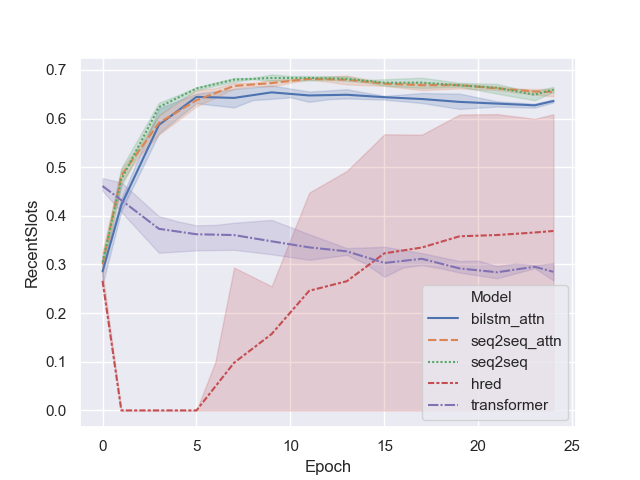}
}
\subfigure[RecentValues]{
    \includegraphics[width=0.8\columnwidth]{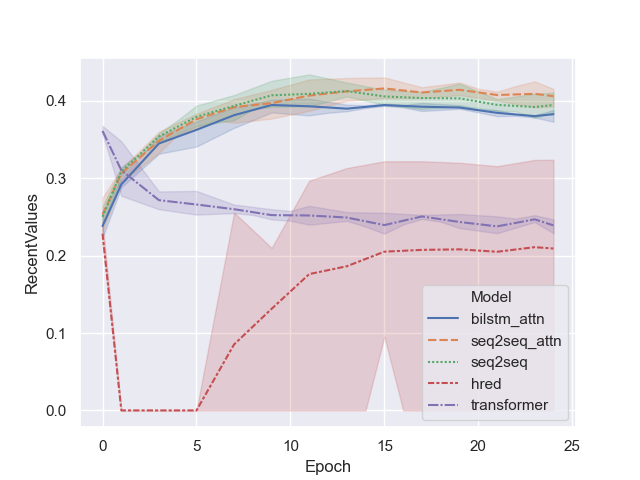}
}
\\
\subfigure[RepeatInfo]{
    \includegraphics[width=0.8\columnwidth]{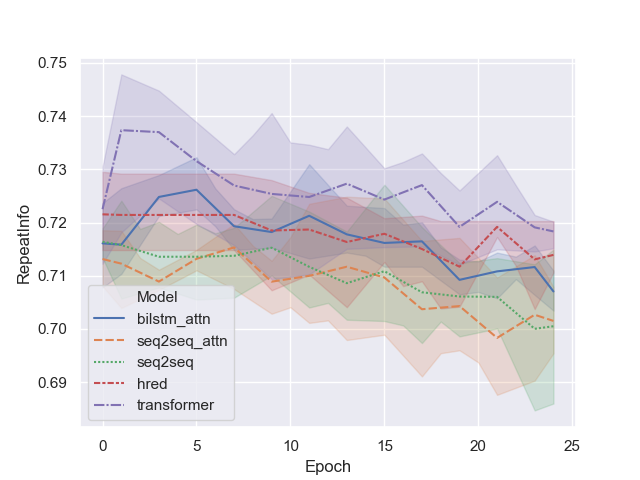}
}
\subfigure[NumRepeatInfo]{
    \includegraphics[width=0.8\columnwidth]{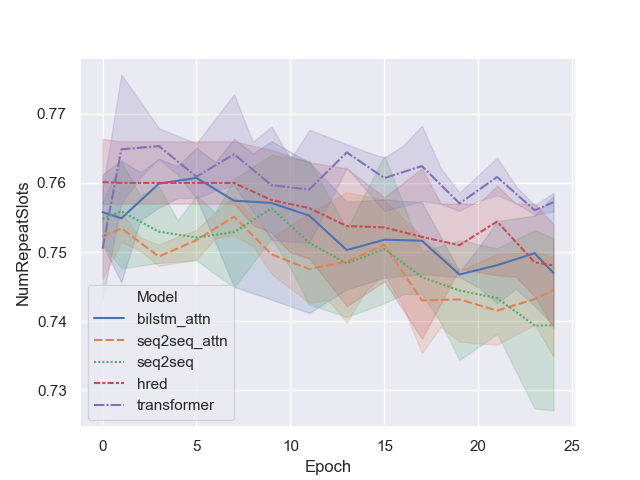}
}
\\
\subfigure[NumRecentInfo]{
    \includegraphics[width=0.8\columnwidth]{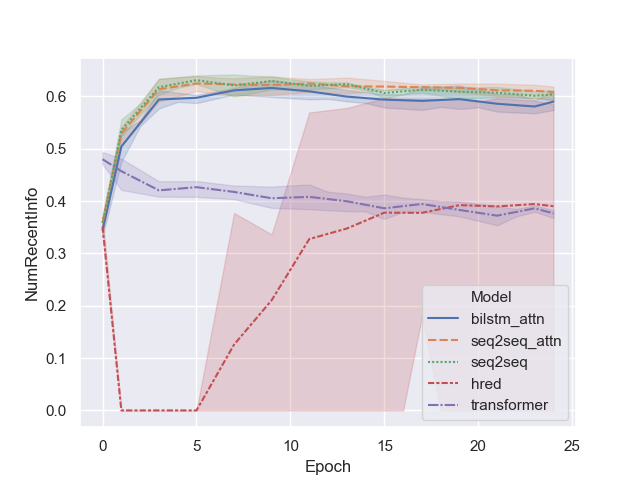}
}
\subfigure[AllSlots]{
    \includegraphics[width=0.8\columnwidth]{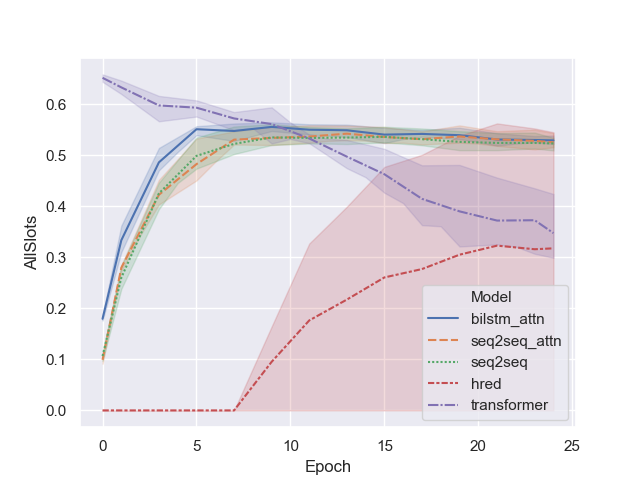}
}

\caption{Progression of performance of models on the probe tasks in MultiWoZ dataset.}
\label{fig:probetasks_table1_multiwoz}
\end{figure*}

\begin{figure*}[h!]
\centering
\subfigure[AllValues]{
    \includegraphics[width=0.8\columnwidth]{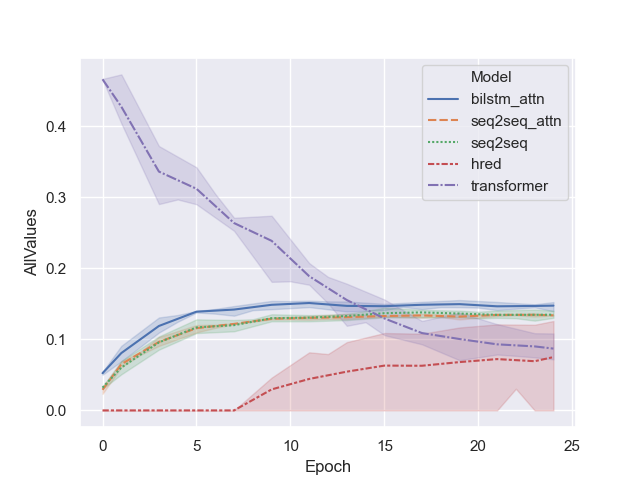}
}
\subfigure[NumAllInfo]{
    \includegraphics[width=0.8\columnwidth]{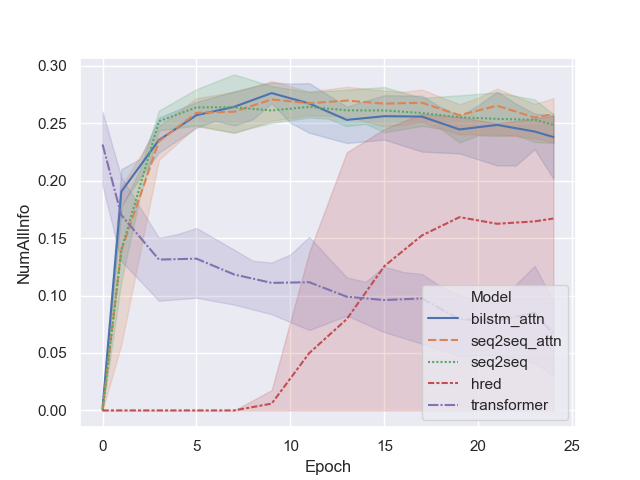}
}
\\
\subfigure[AllTopics]{
    \includegraphics[width=0.8\columnwidth]{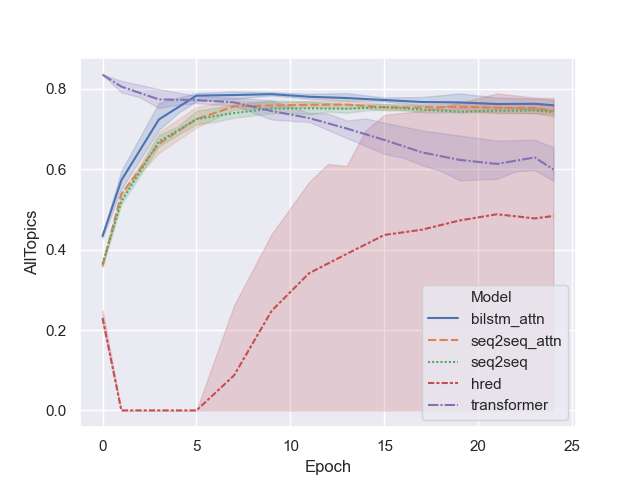}
}
\subfigure[RecentValues]{
    \includegraphics[width=0.8\columnwidth]{Images/Analysis/plot_RecentValues.png}
}
\\
\subfigure[NumAllTopics]{
    \includegraphics[width=0.8\columnwidth]{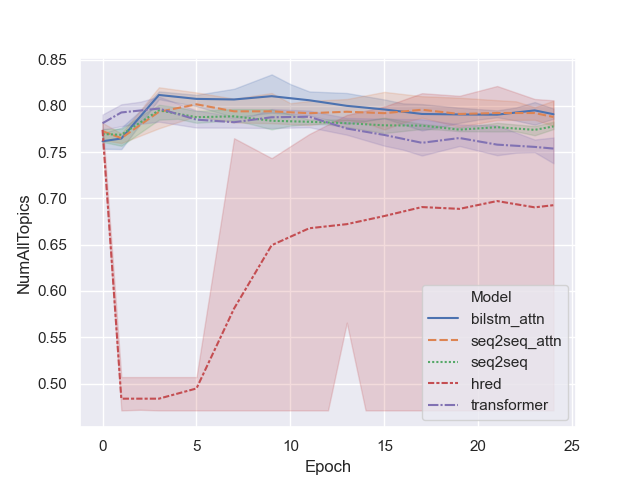}
}
\subfigure[IsMultiTask]{
    \includegraphics[width=0.8\columnwidth]{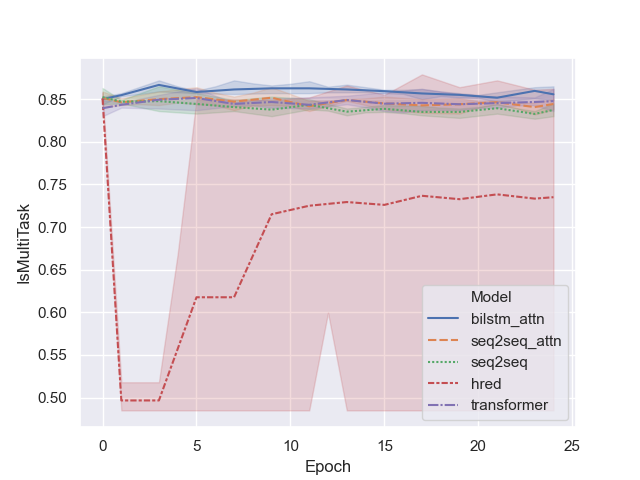}
}
\\
\subfigure[EntitySlots]{
    \includegraphics[width=0.8\columnwidth]{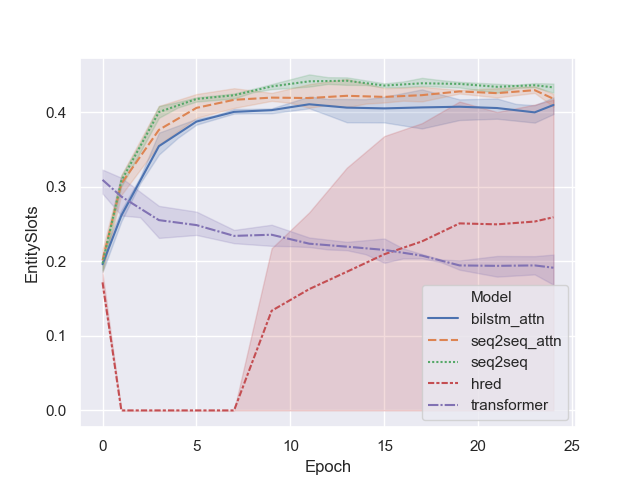}
}
\subfigure[EntityValues]{
    \includegraphics[width=0.8\columnwidth]{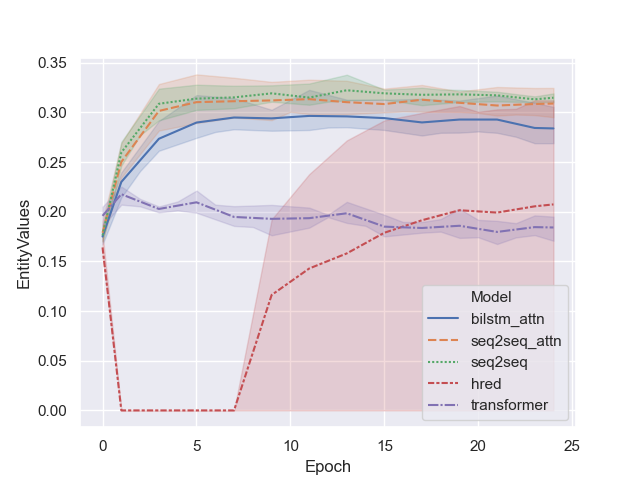}
}

\caption{Progression of performance of models on the probe tasks in MultiWoZ dataset.}
\label{fig:probetasks_table2_multiwoz}
\end{figure*}

\begin{figure*}[h!]
\centering
\subfigure[UtteranceLoc]{
    \includegraphics[width=0.8\columnwidth]{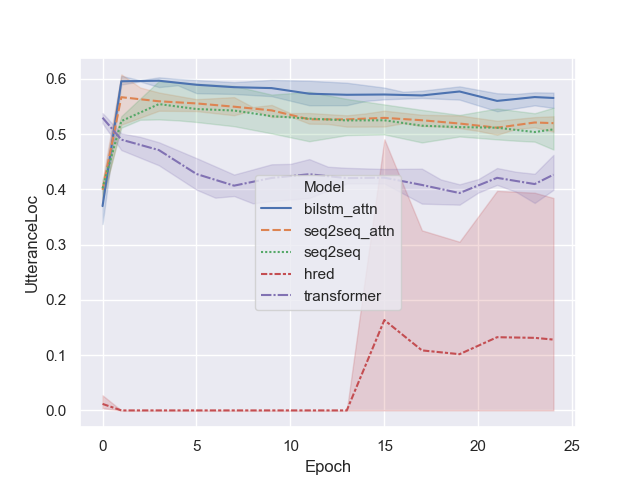}
}
\subfigure[WordCont]{
    \includegraphics[width=0.8\columnwidth]{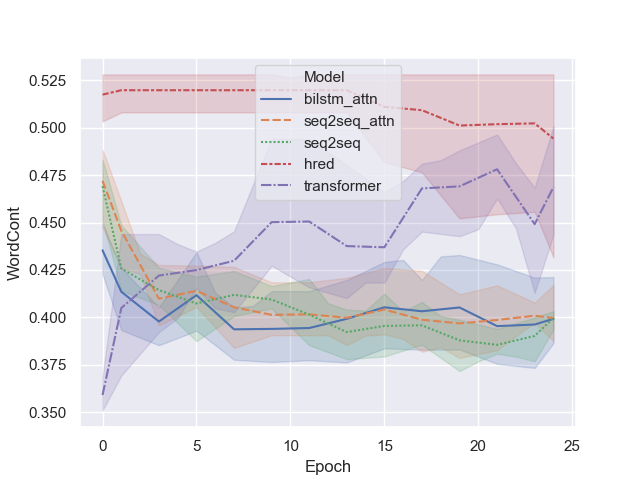}
}
\subfigure[PersonalInfo]{
    \includegraphics[width=0.8\columnwidth]{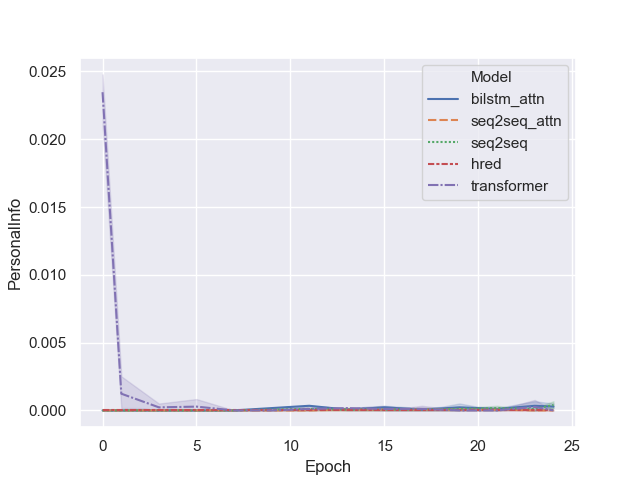}
}
\caption{Progression of performance of models on the probe tasks in PersonaChat dataset.}
\label{fig:probetasks_table1_personachat}
\end{figure*}

\section{Human Evaluation Details}

We collected human annotation on comparing the relevance between two responses from the same model architecture but with different seeds. We used ParlAI's mturk framework to set up our human evaluation (Figure \ref{fig:human_eval_examples}). 

We provide the users a detailed set of instructions on relevance of the generated text with four different examples. On top of that, we start the data collection with a few sanity check questions (the participant is not told that it is a test question) where the correct answers were obvious. When the participant failed thrice, we soft block them and do not allow them to participate in our data collection. 

With this set up, we collected data only from 508 participants out of 1004 who took the sanity check task. This ensured the quality of the data collected.

\begin{figure*}[h!]
\centering
\subfigure[Example1]{
    \includegraphics[width=0.8\columnwidth]{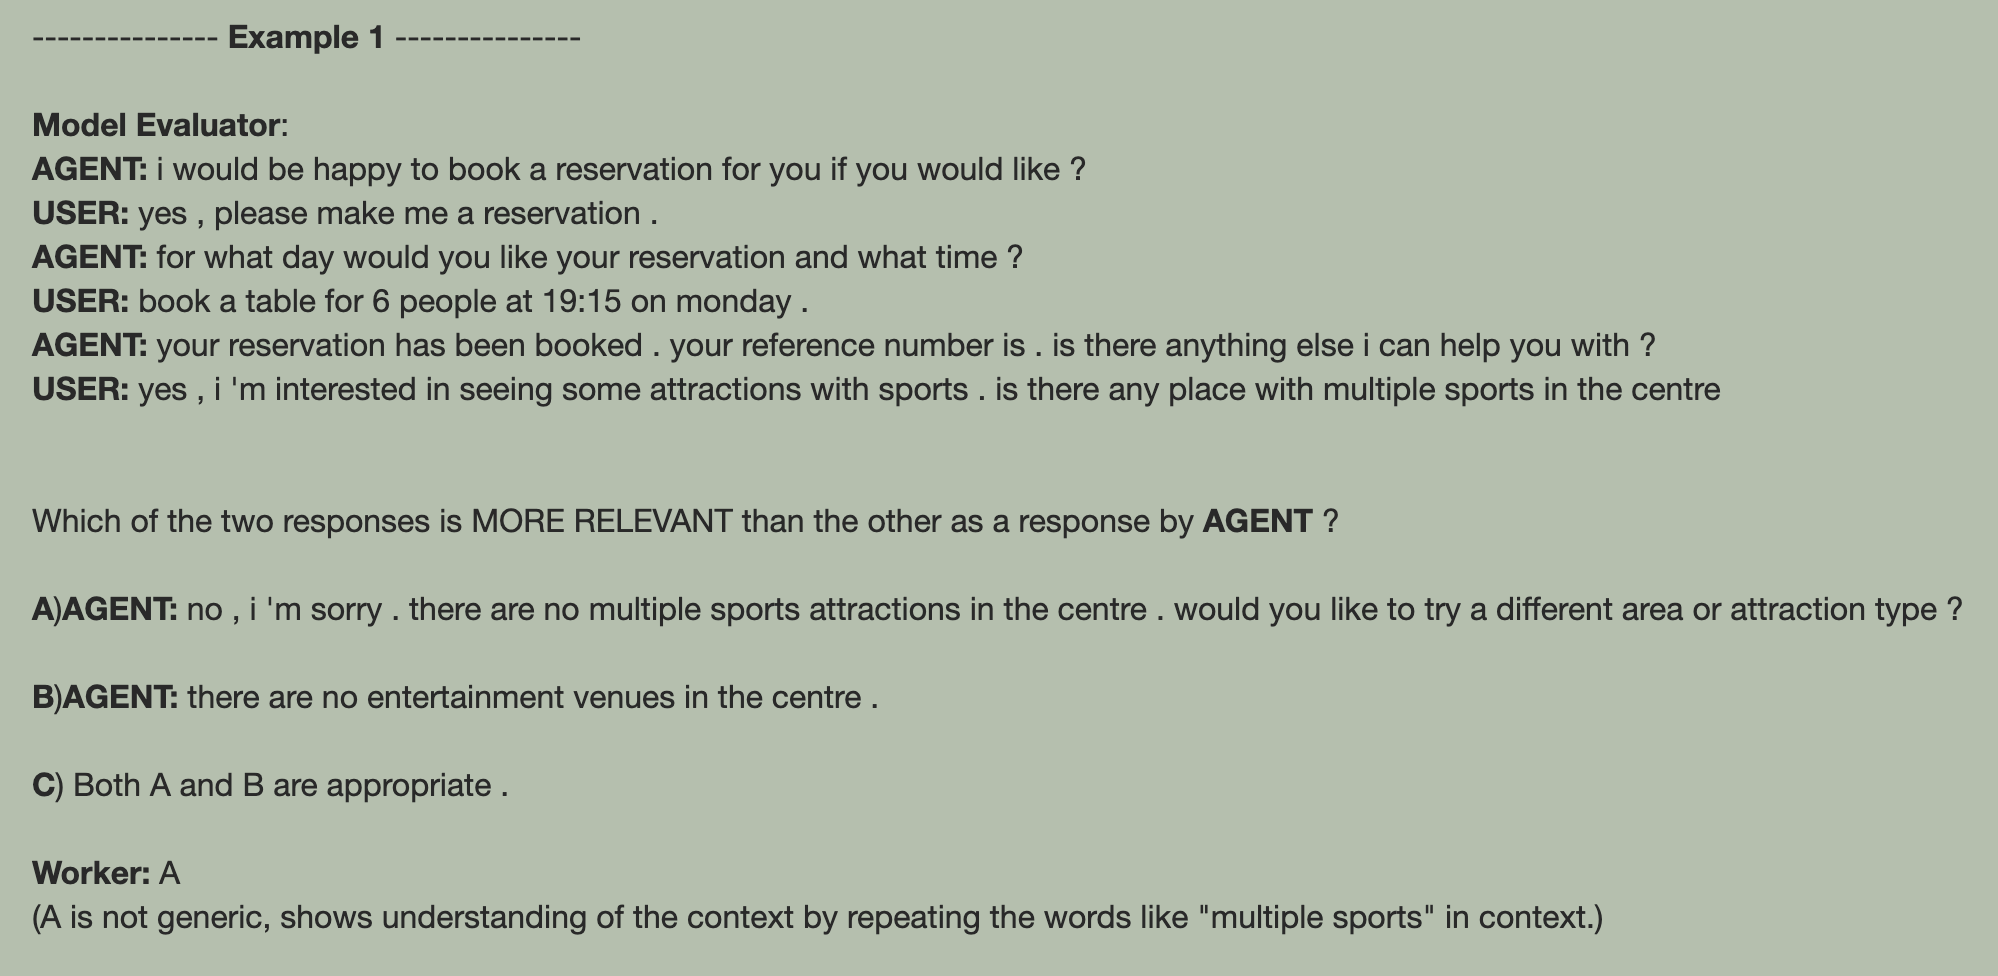}
}
\subfigure[Example2]{
    \includegraphics[width=0.8\columnwidth]{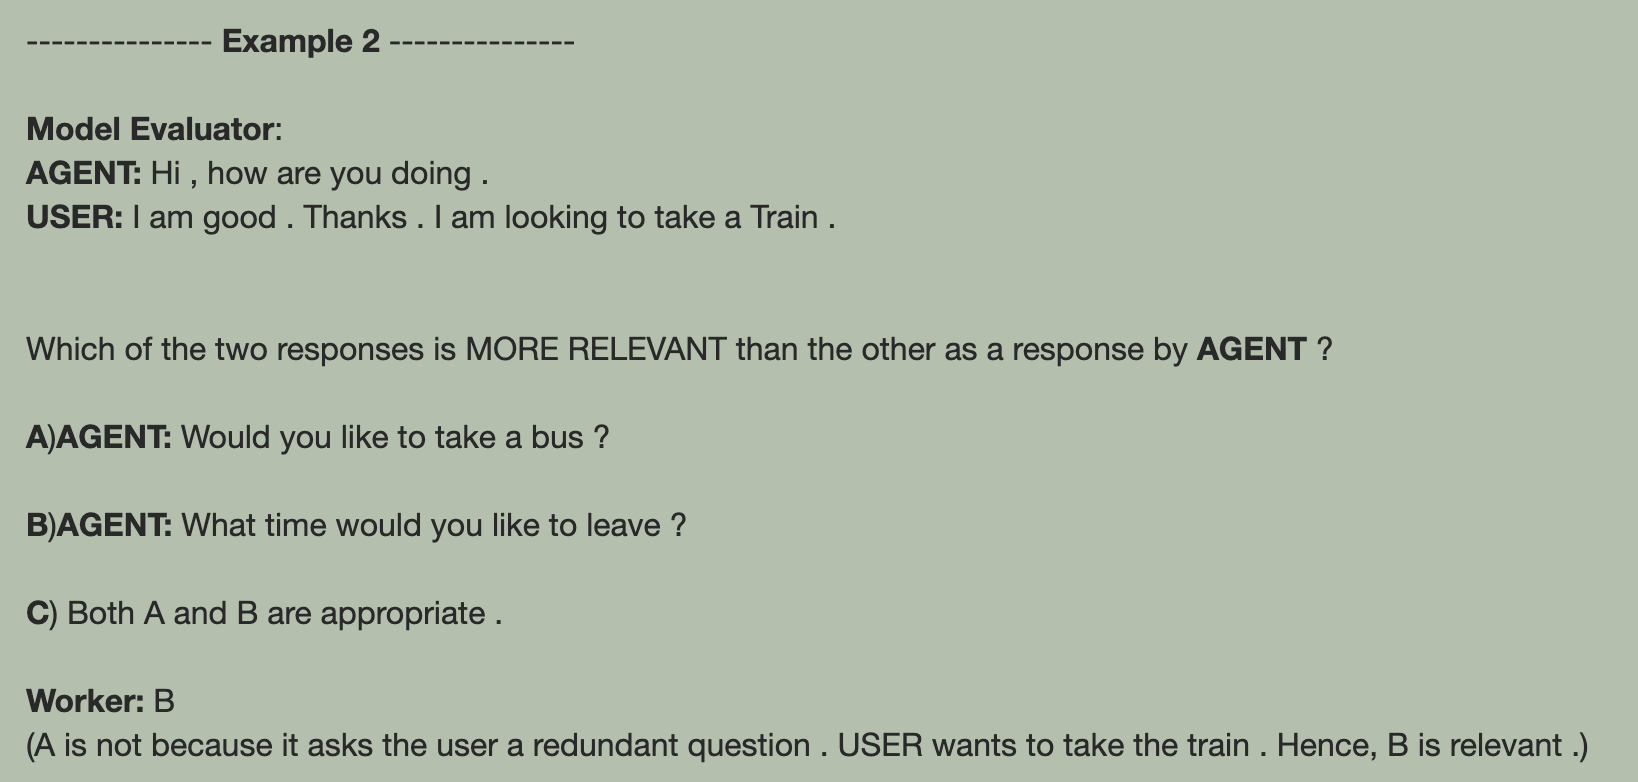}
}
\\
\subfigure[Example3]{
    \includegraphics[width=0.8\columnwidth]{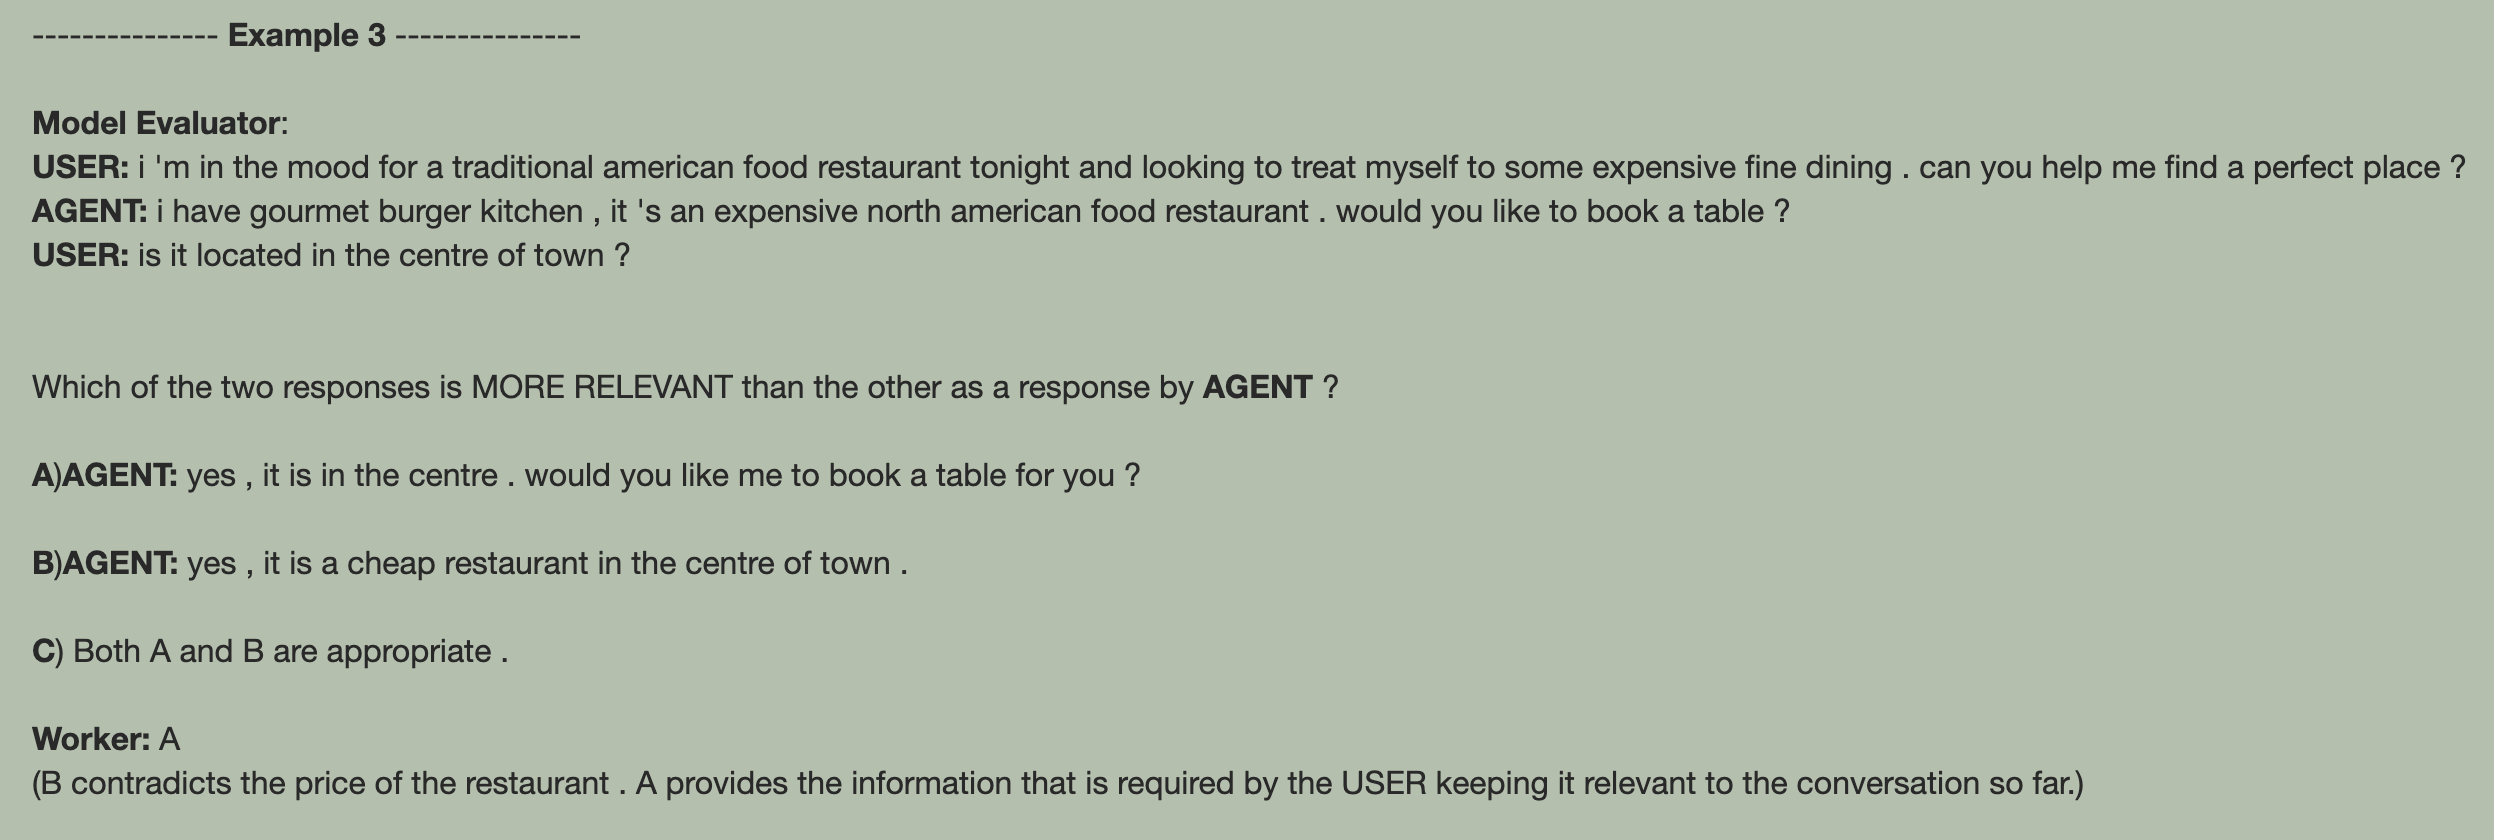}
}
\subfigure[Example4]{
    \includegraphics[width=0.8\columnwidth]{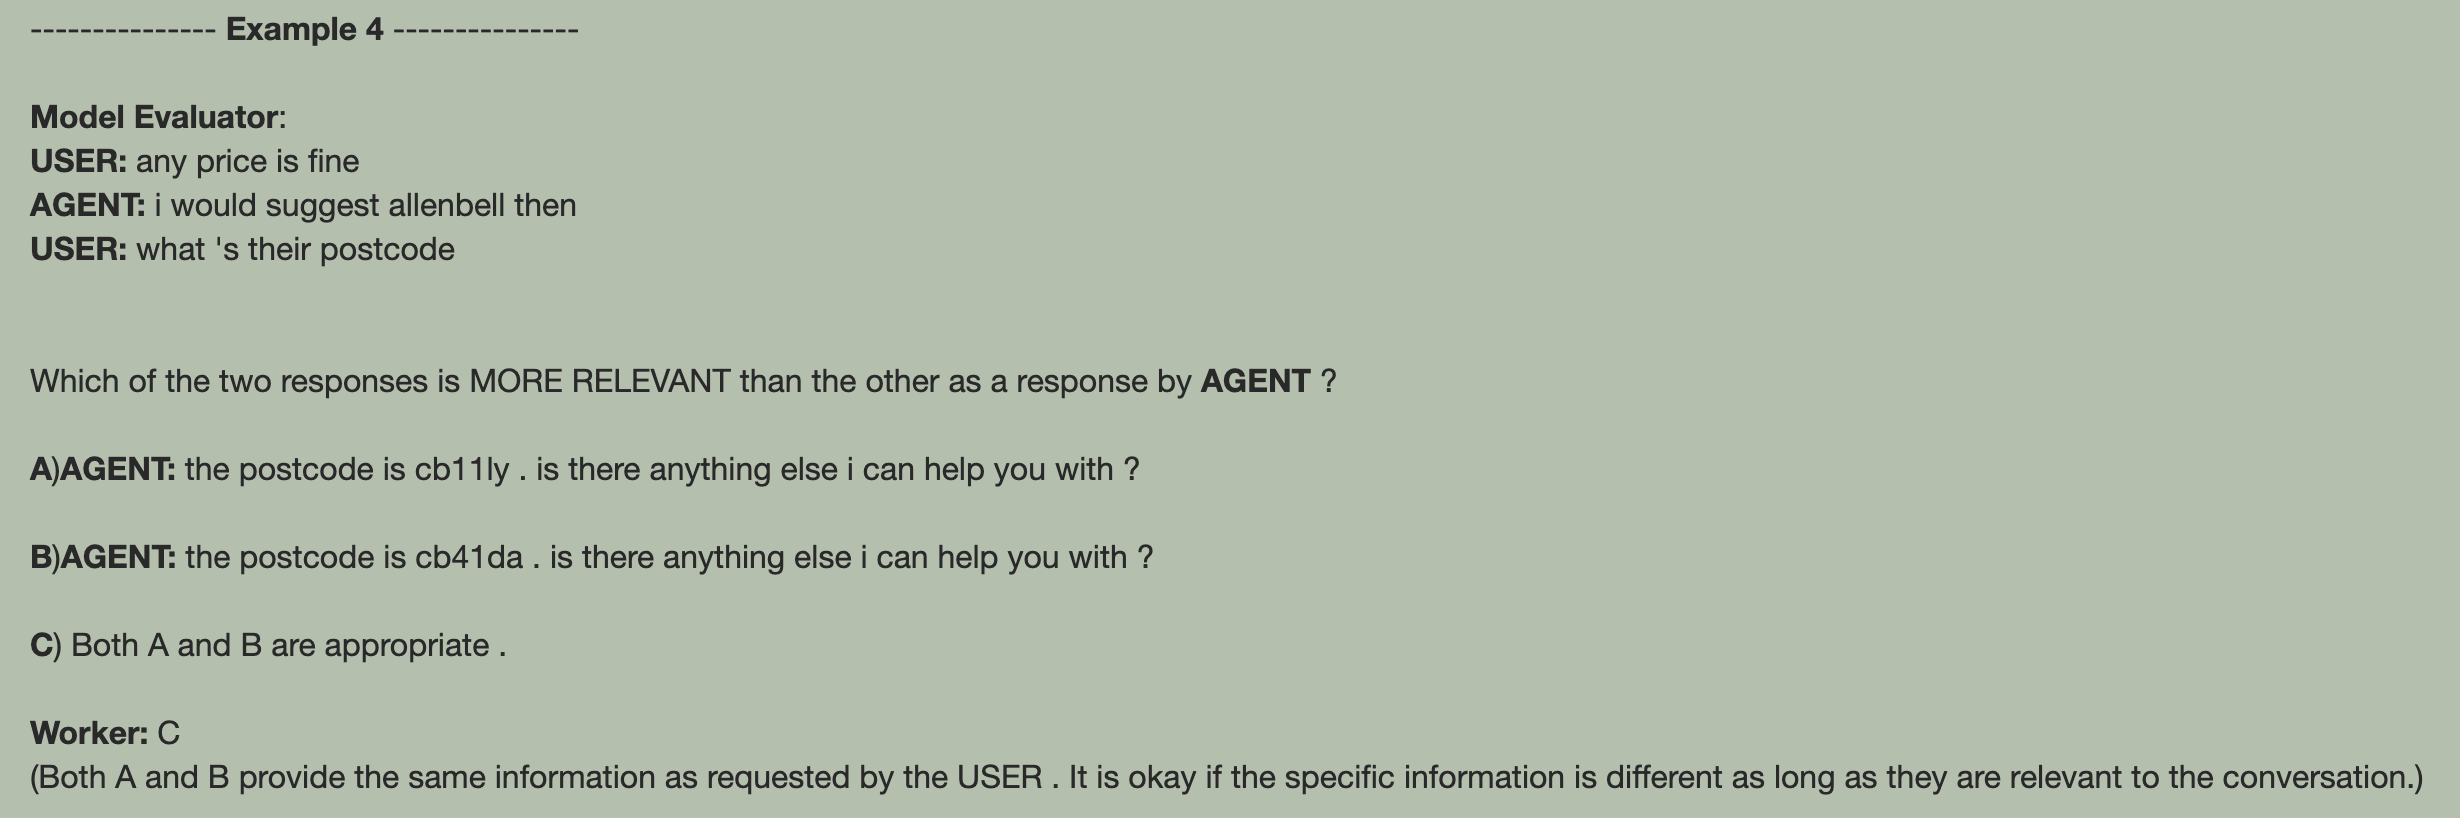}
}
\\
\subfigure[General Instruction]{
    \includegraphics[width=0.8\columnwidth]{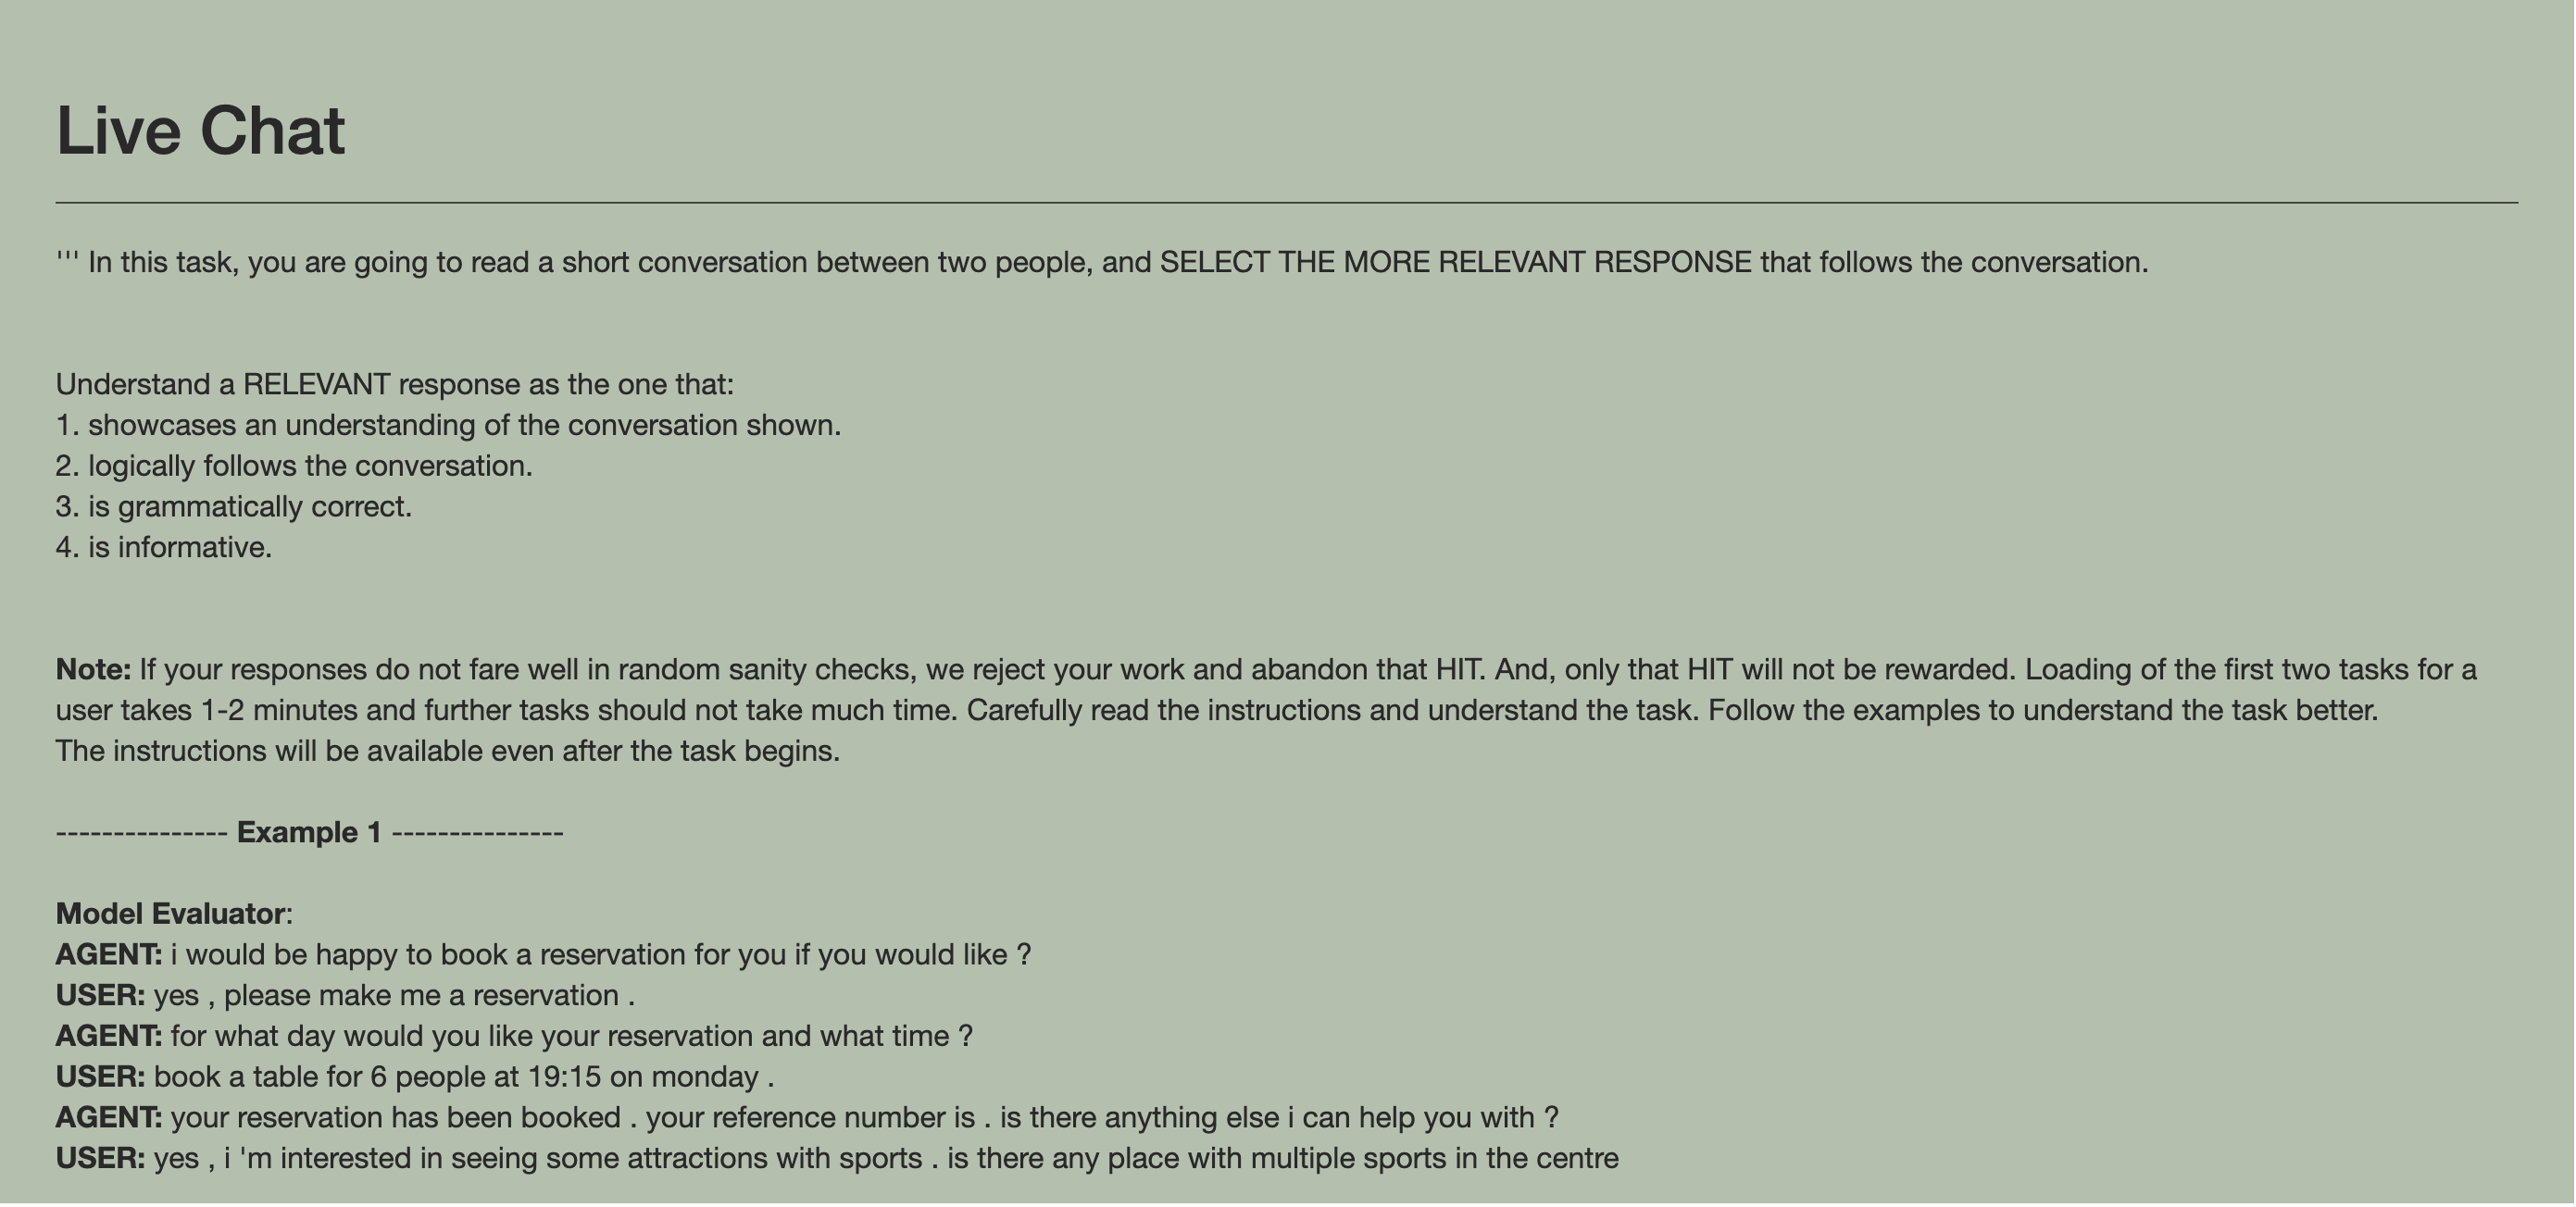}
}
\subfigure[HIT]{
    \includegraphics[width=0.8\columnwidth]{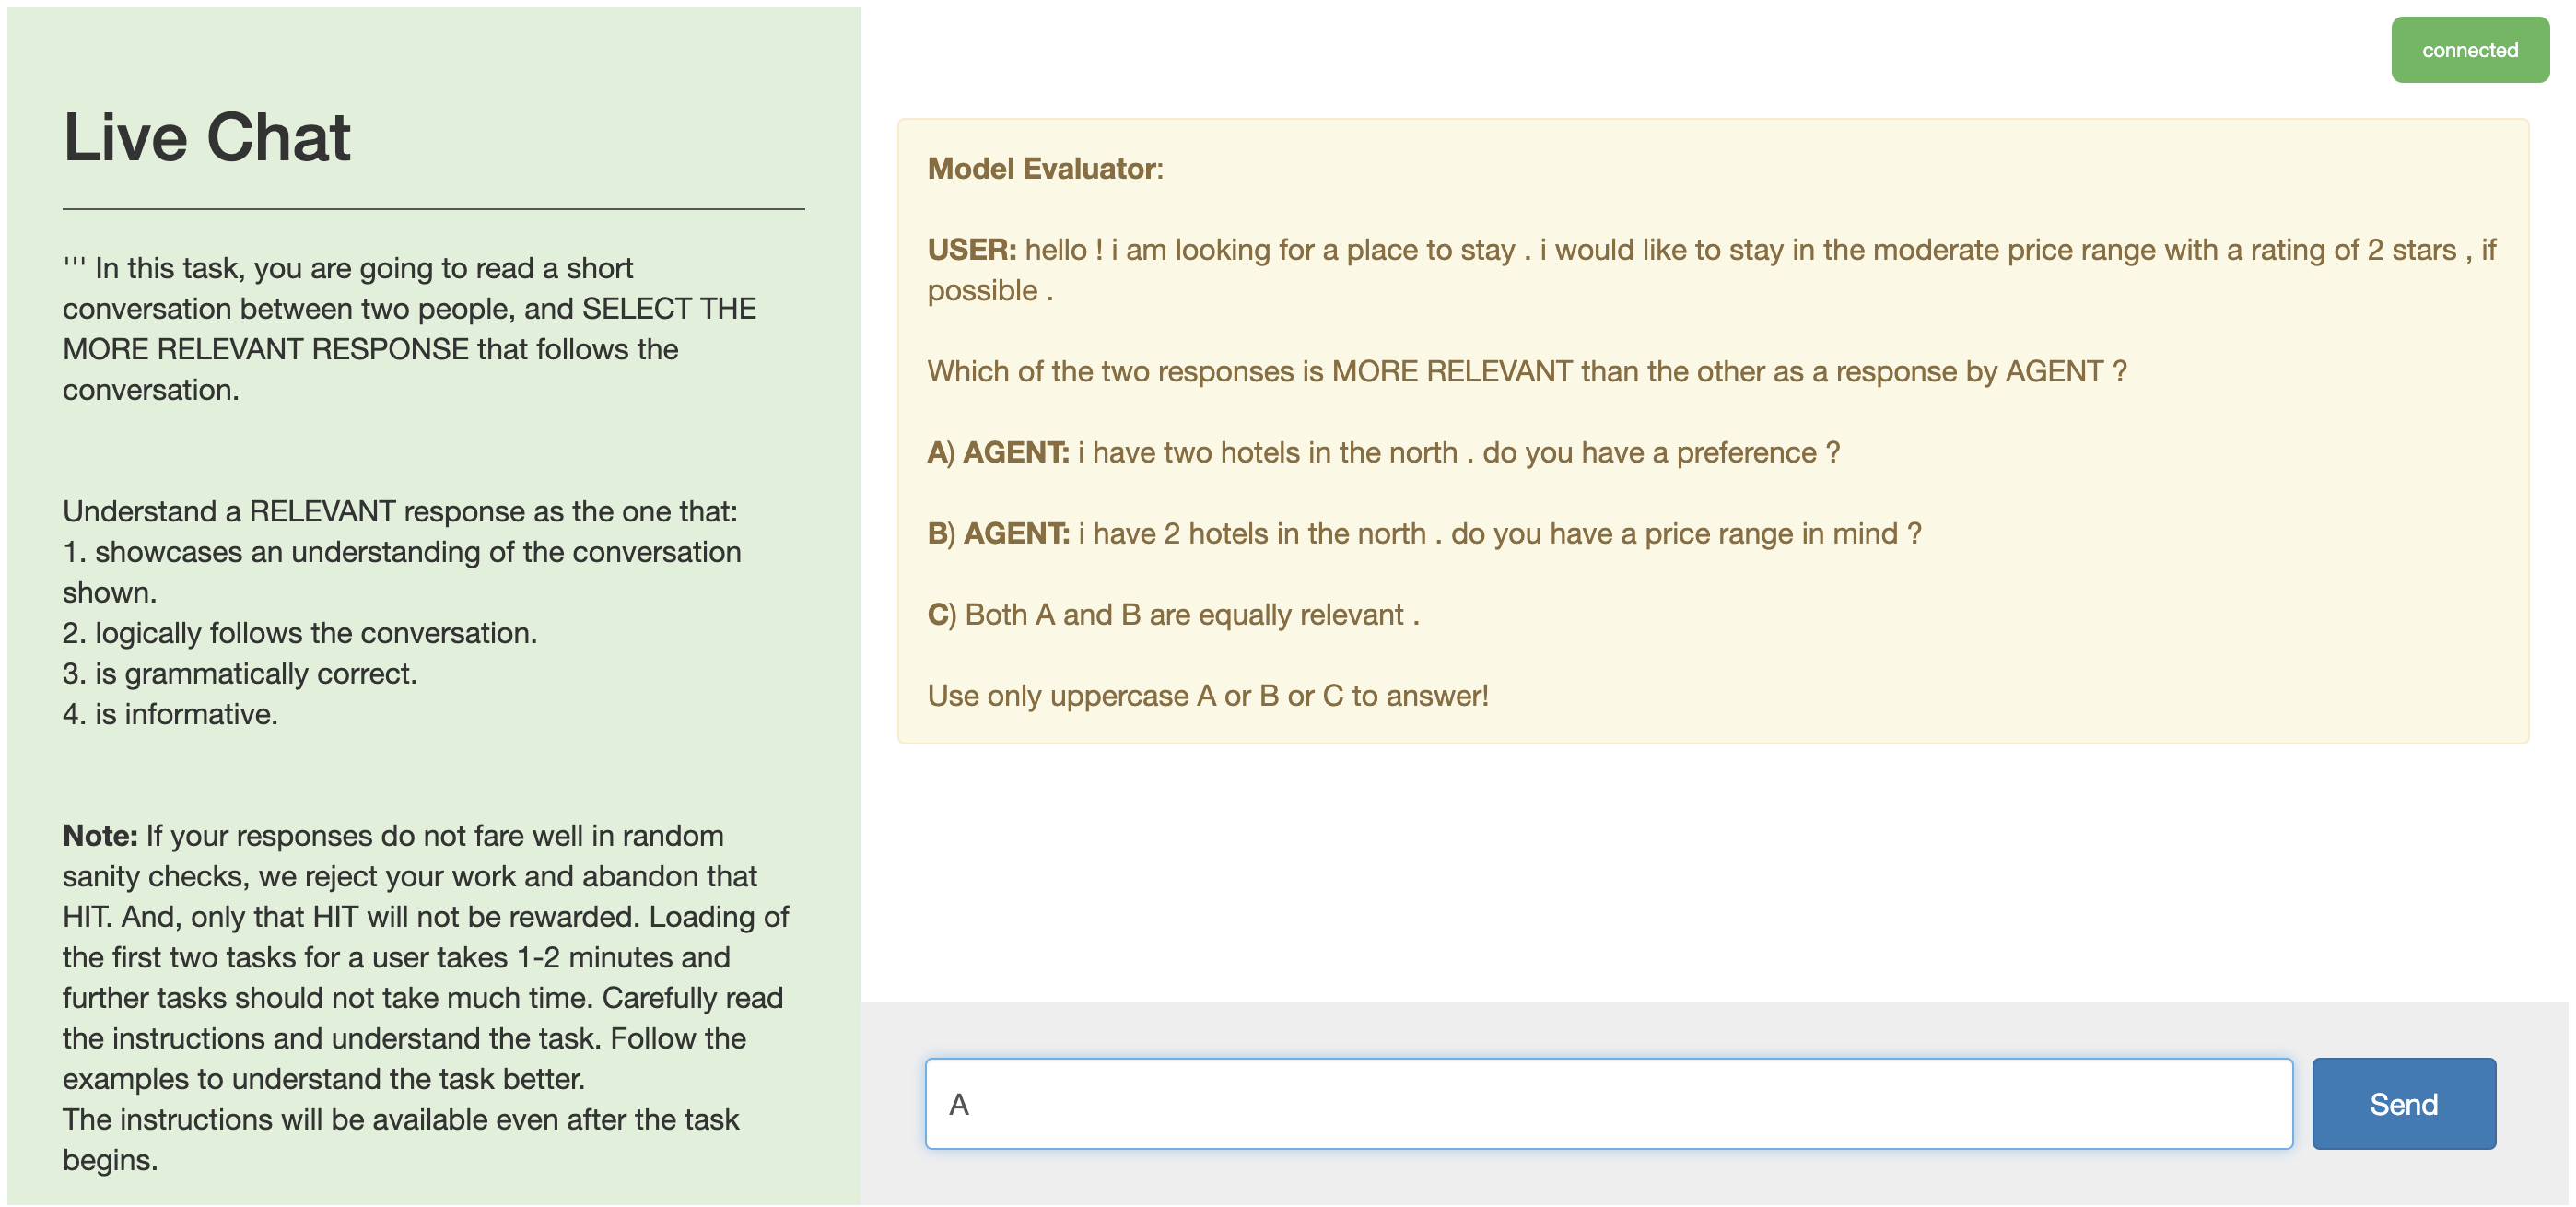}
}
\caption{Examples used to illustrate the nature of the task for data collection with ParlAI and Amazon Mechanical Turk.}
\label{fig:human_eval_examples}
\end{figure*}
